# Supplementary material for: FocDepthFormer: Transformer with latent LSTM for Depth Estimation from Focal Stack
Source: arXiv:2310.11178 source file (2024-12-04)

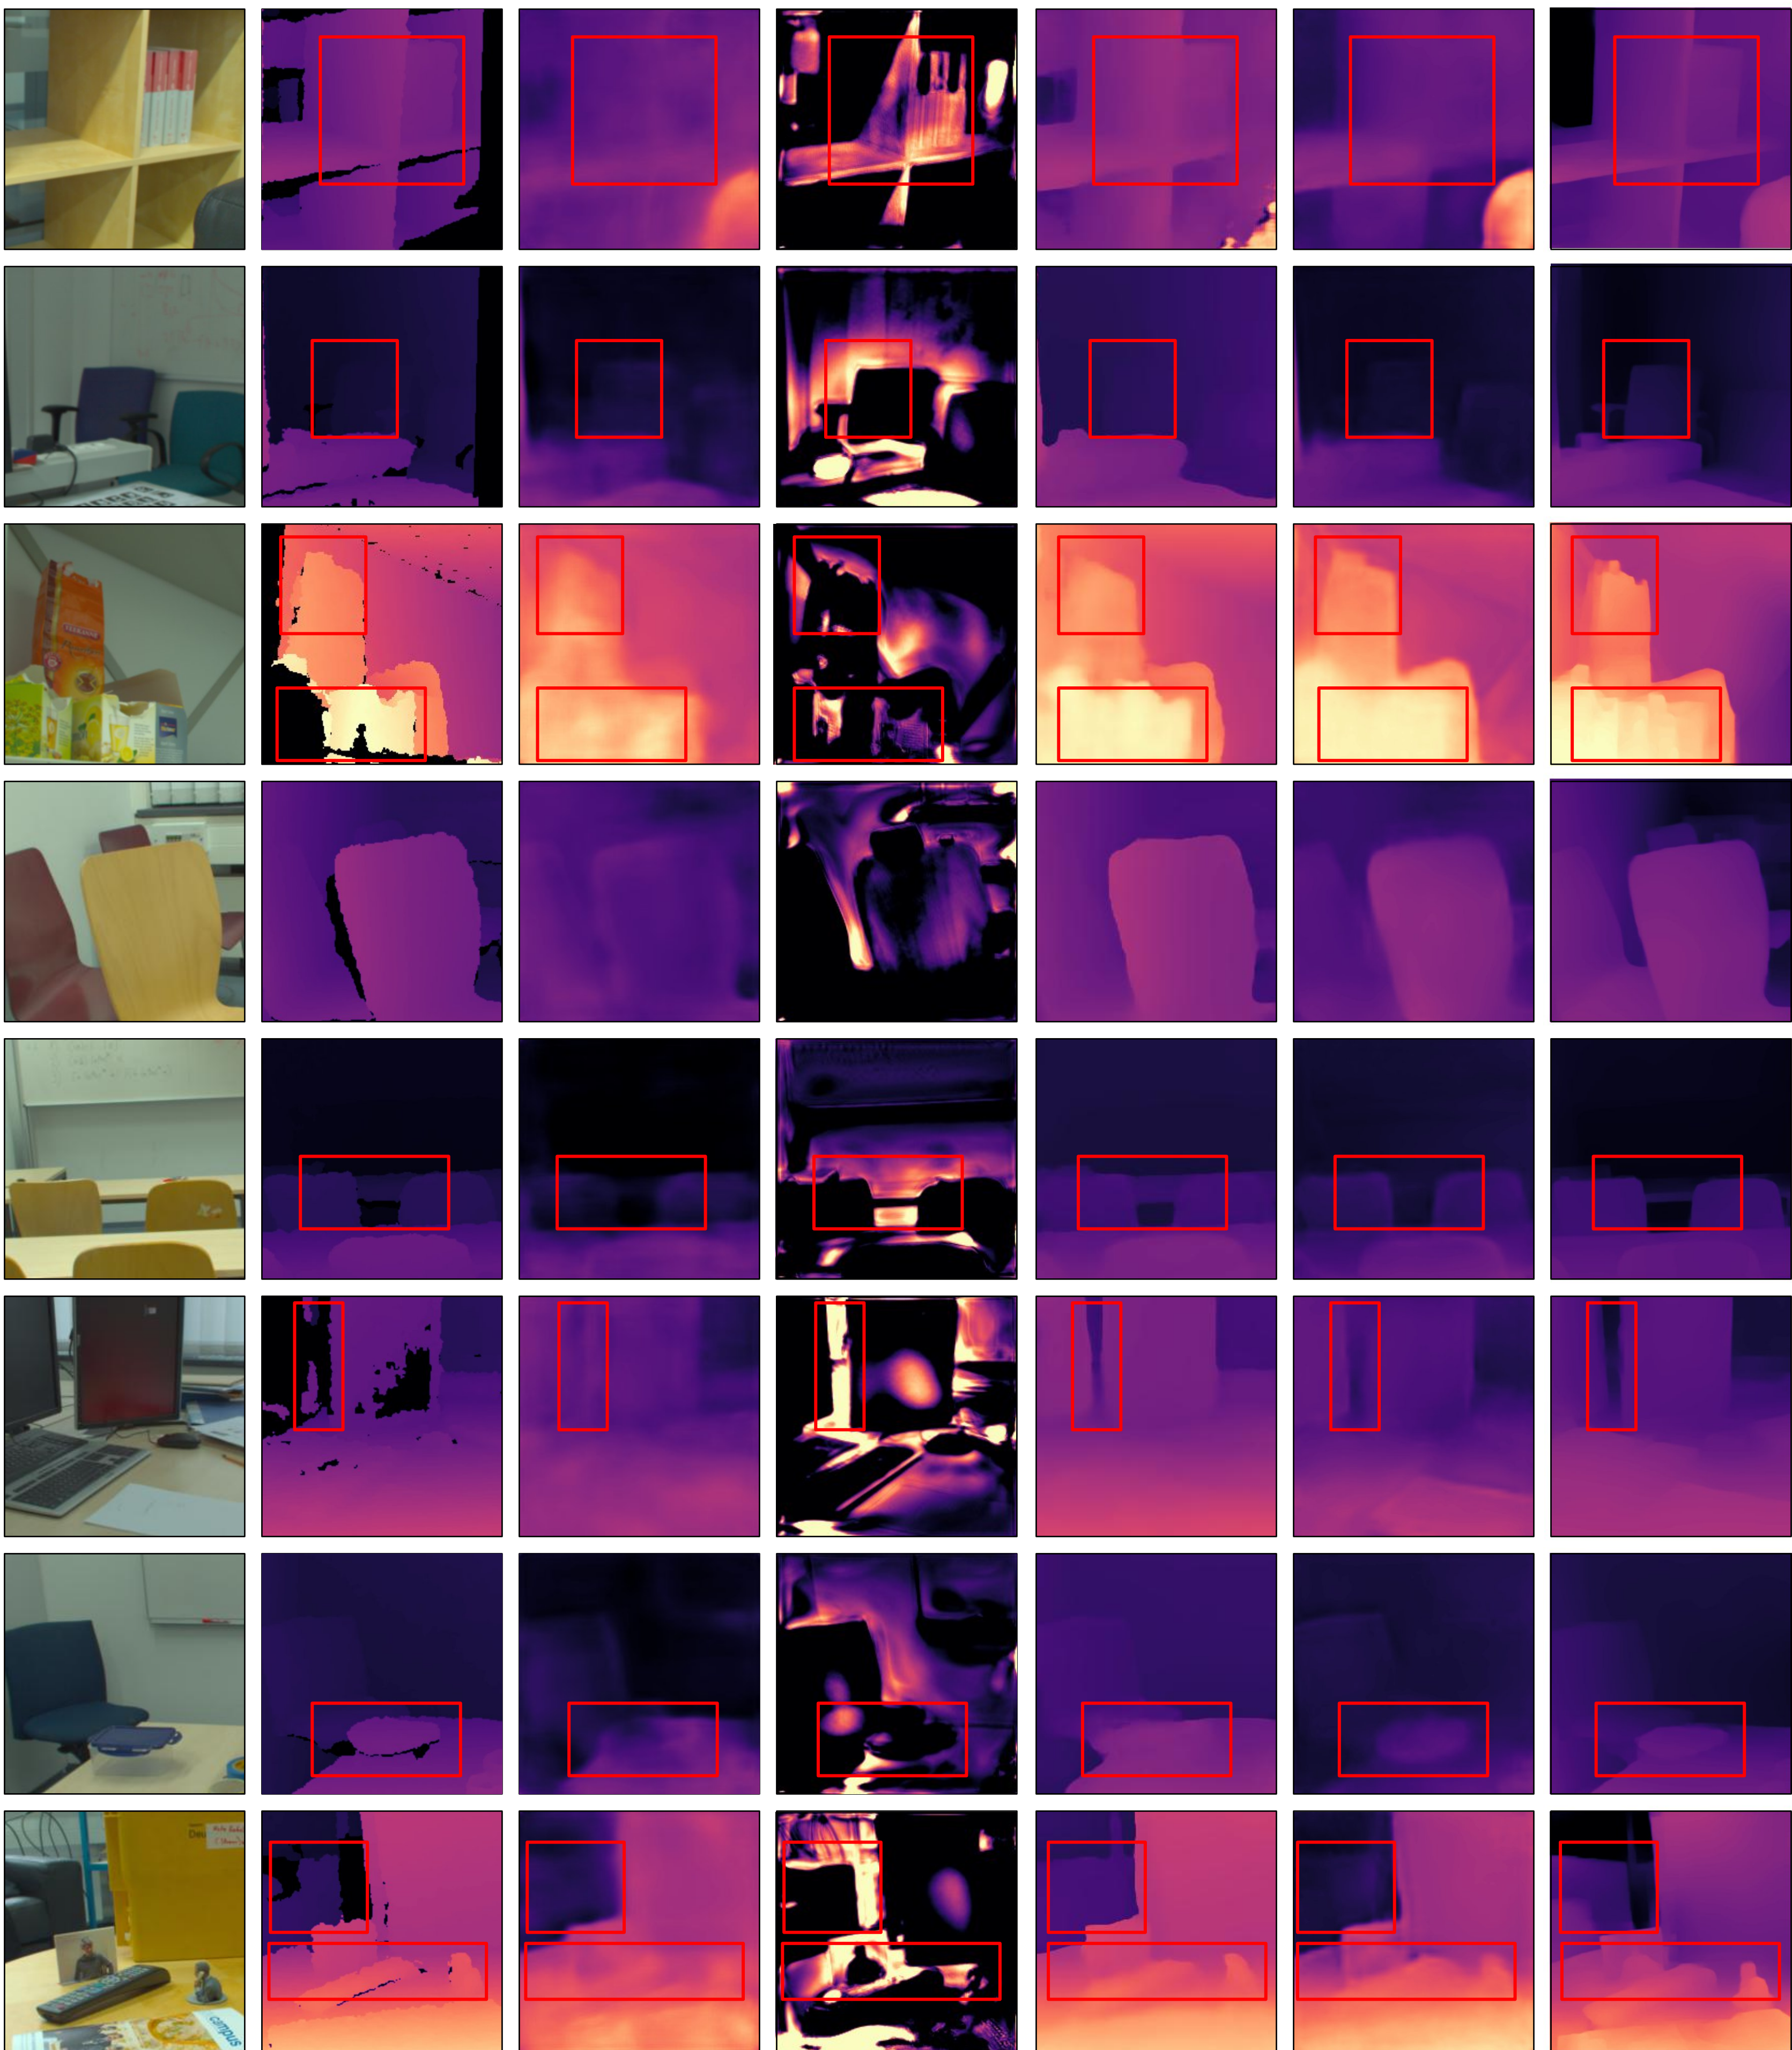



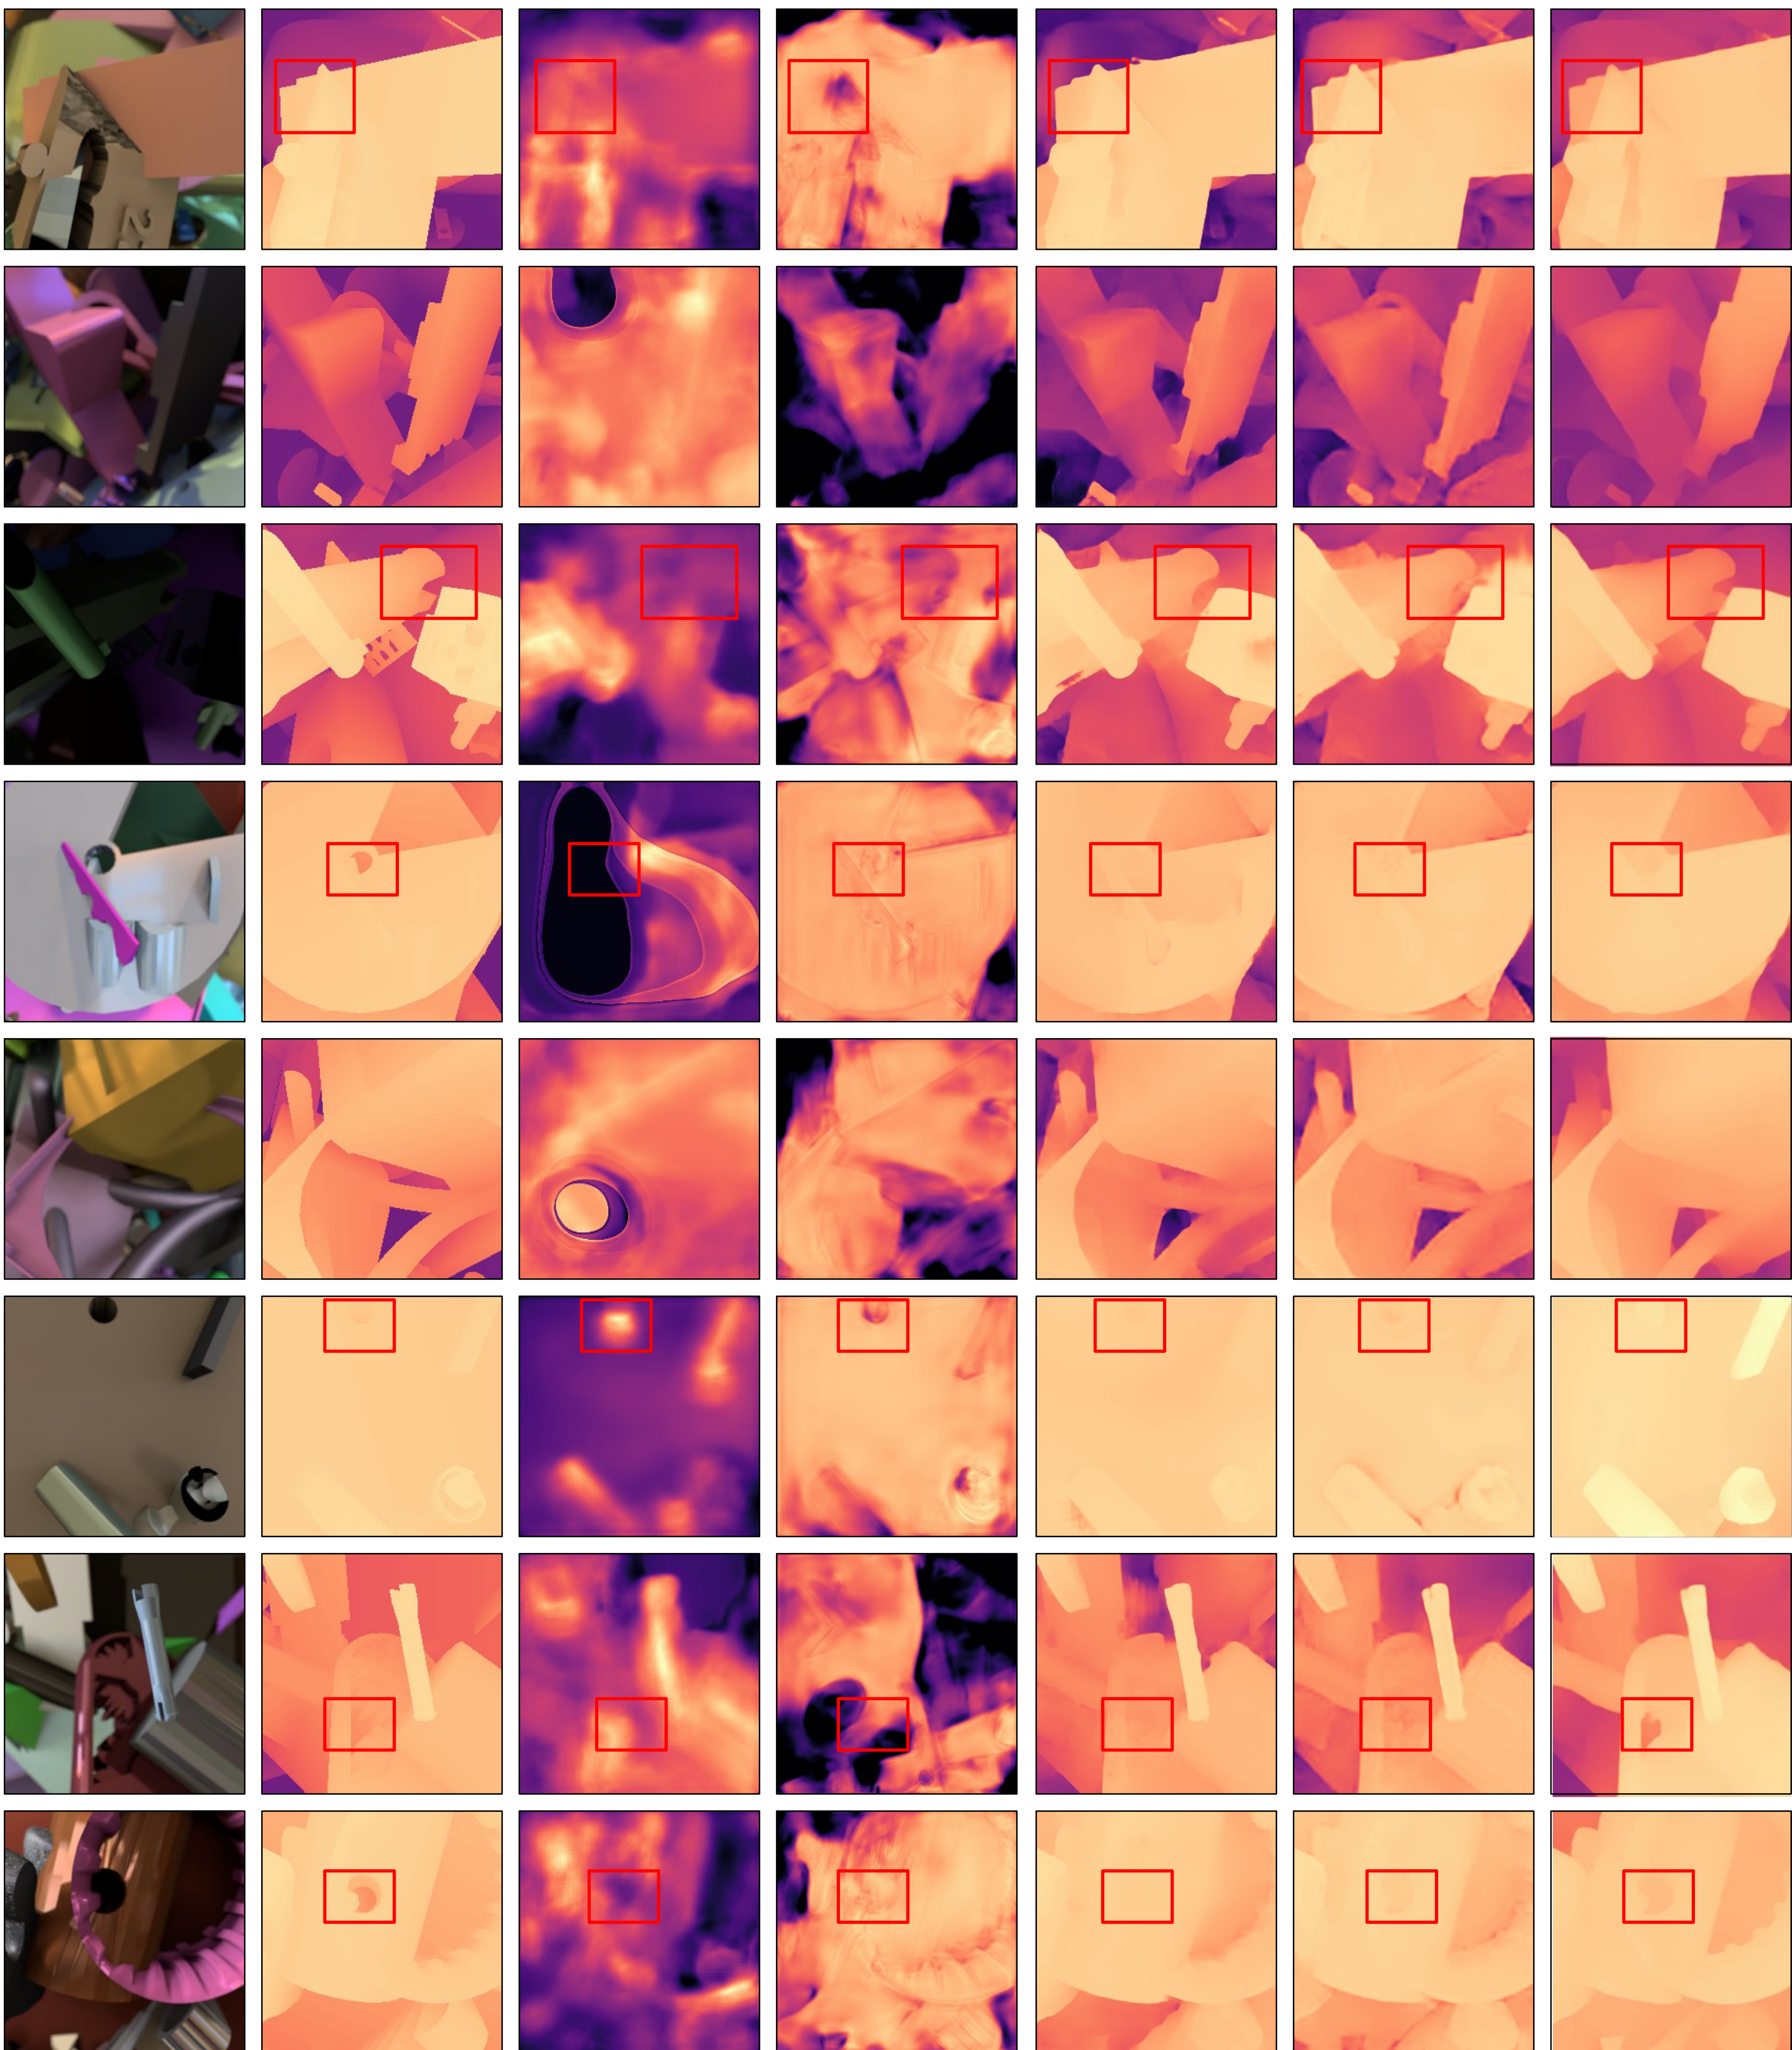



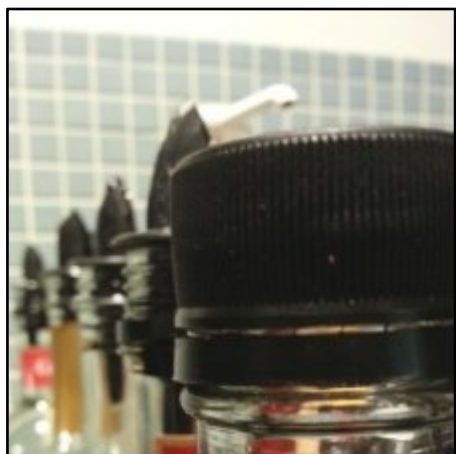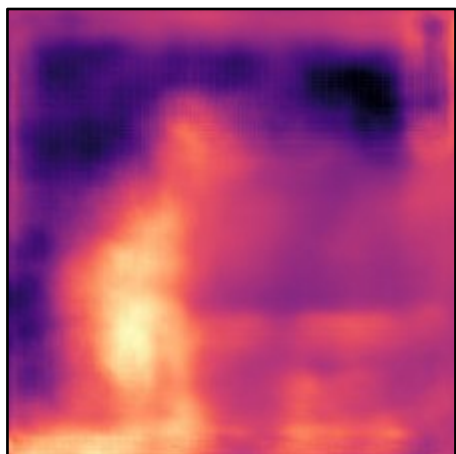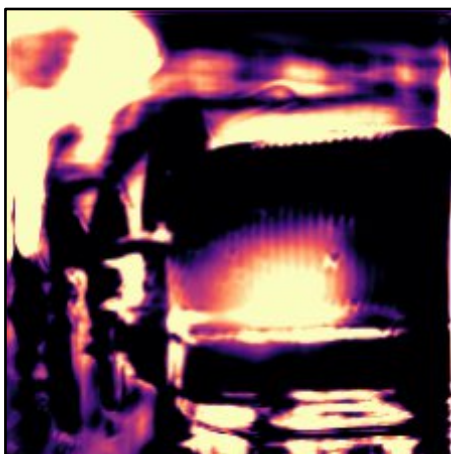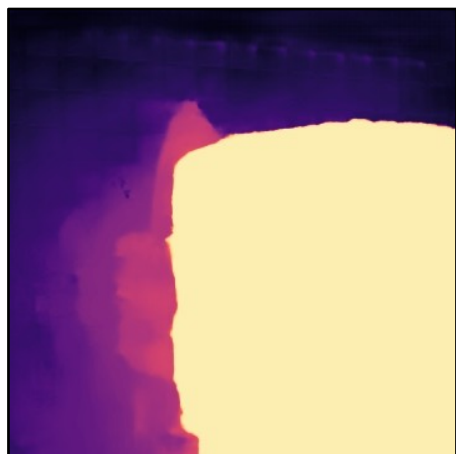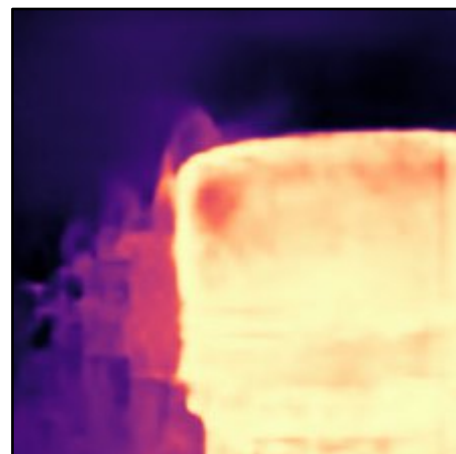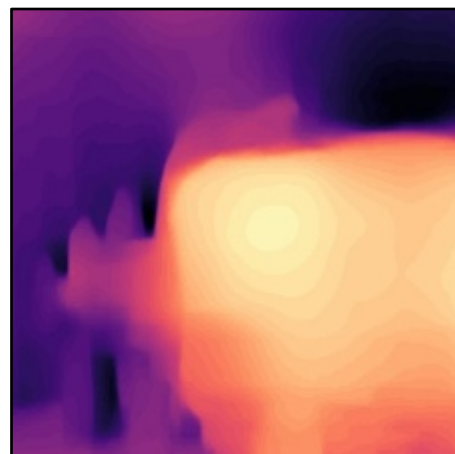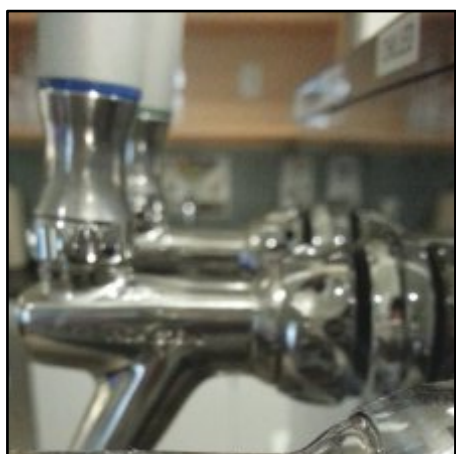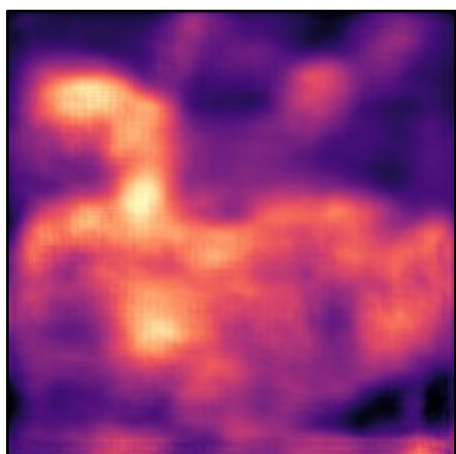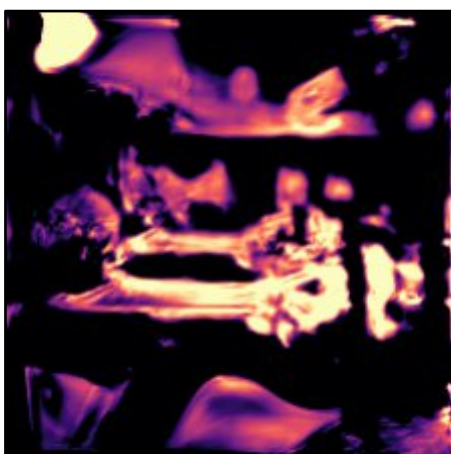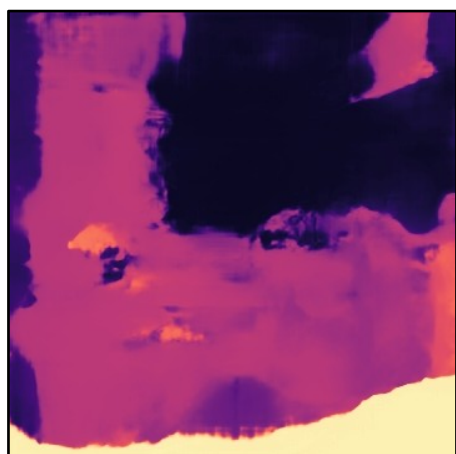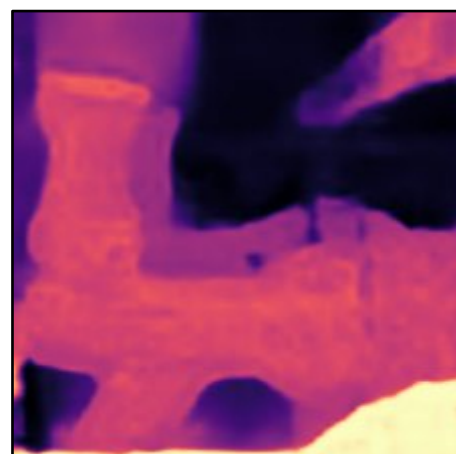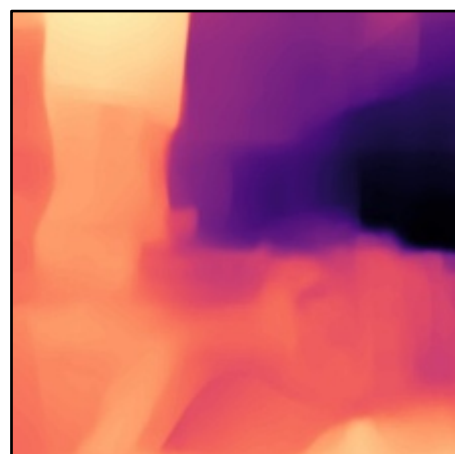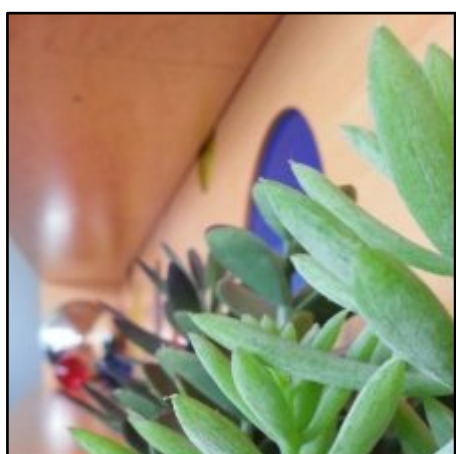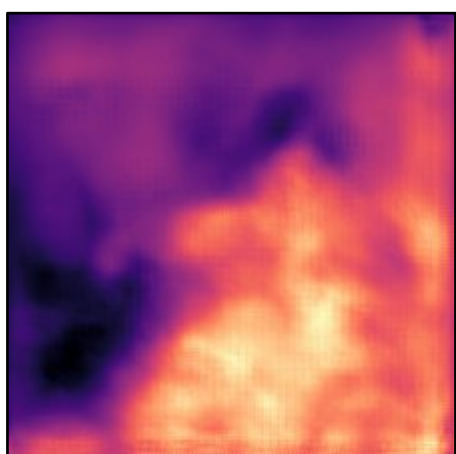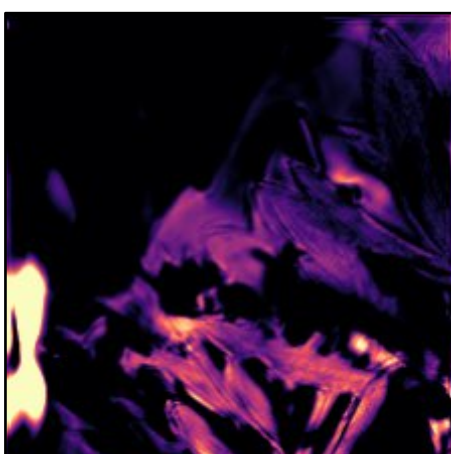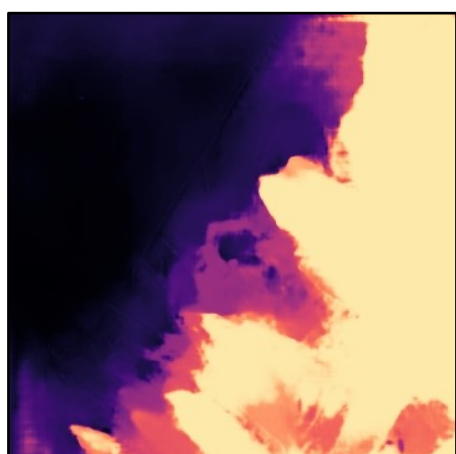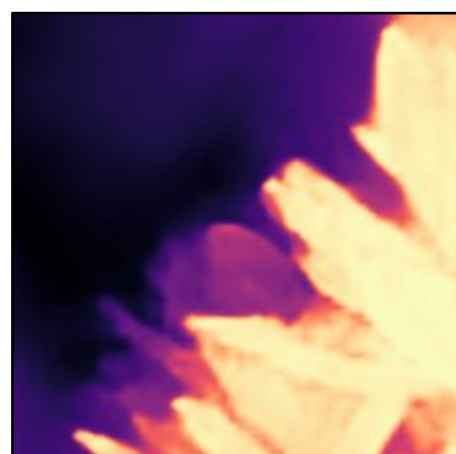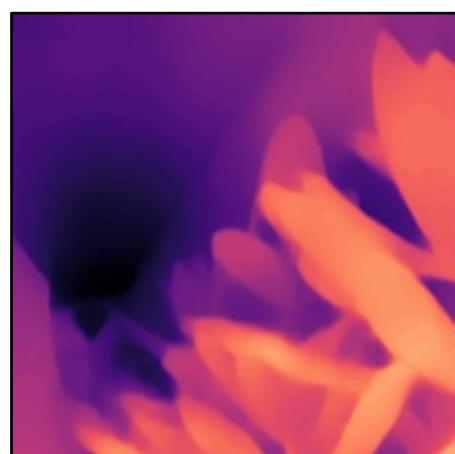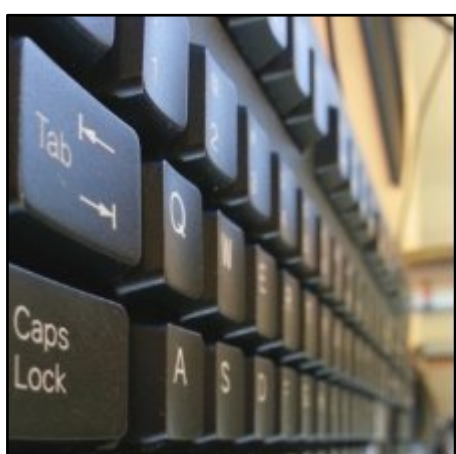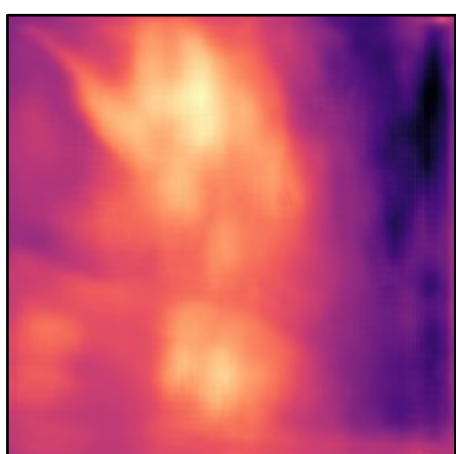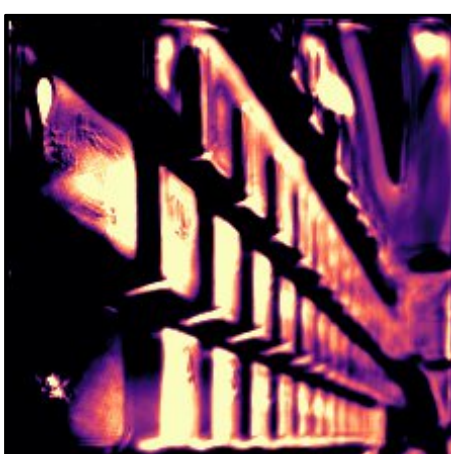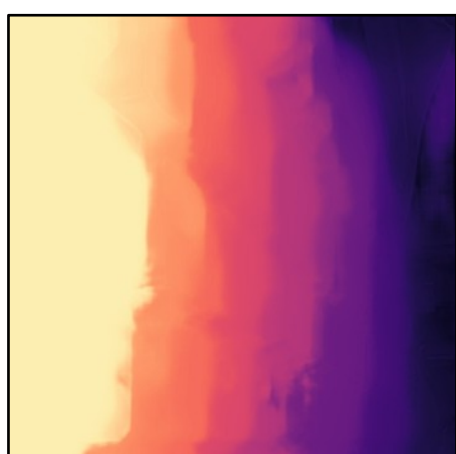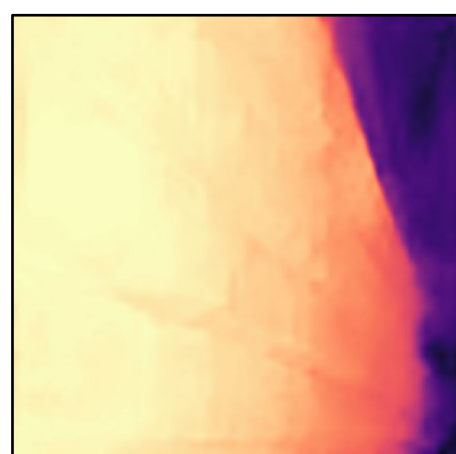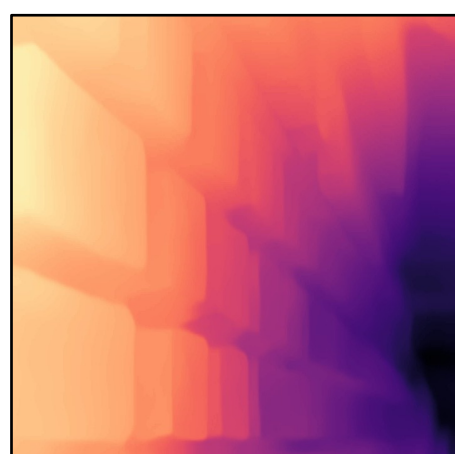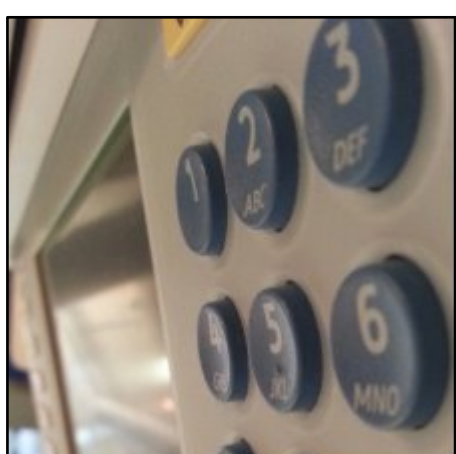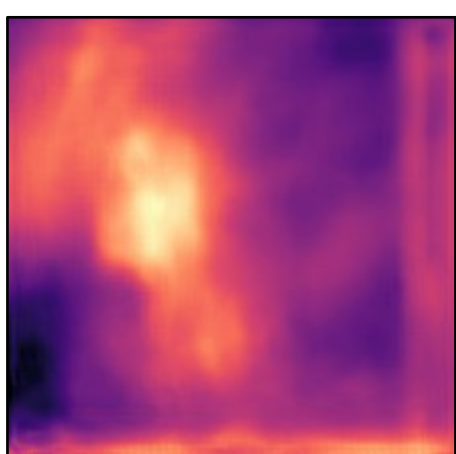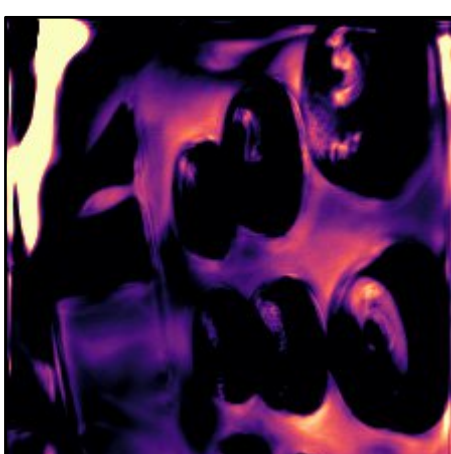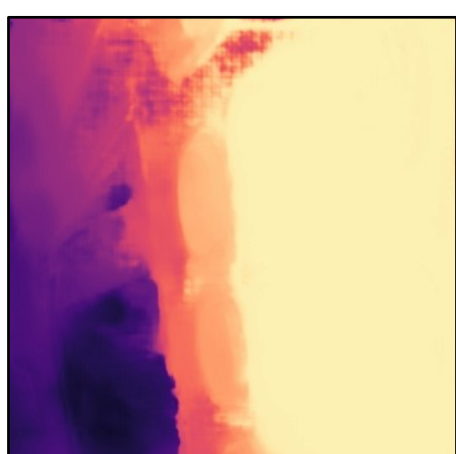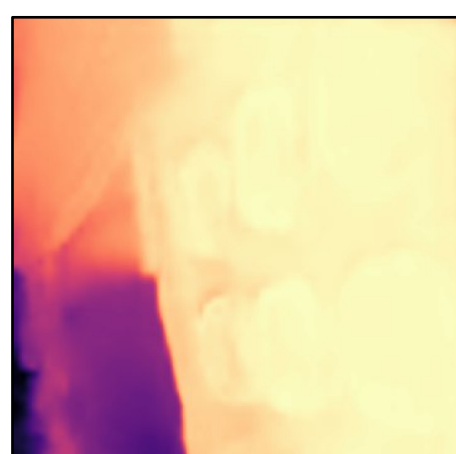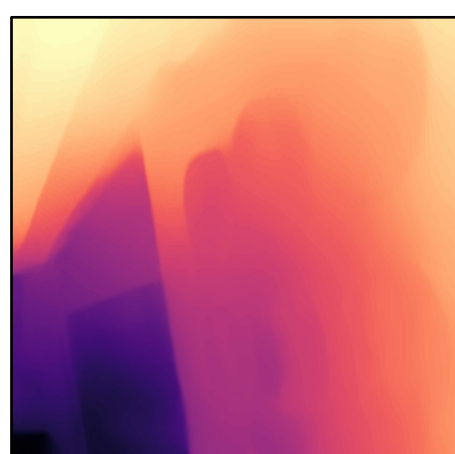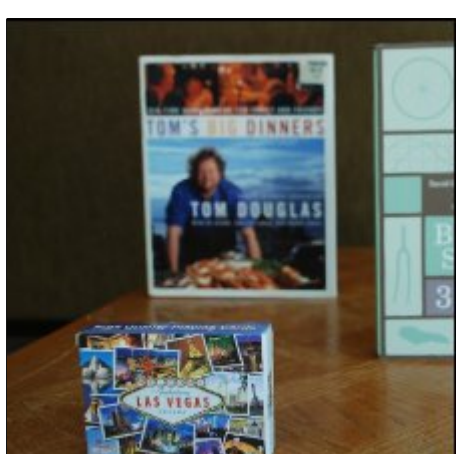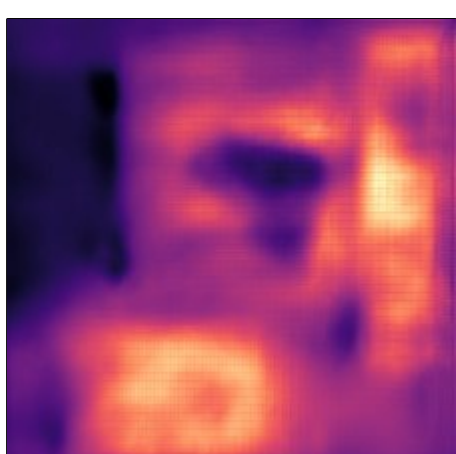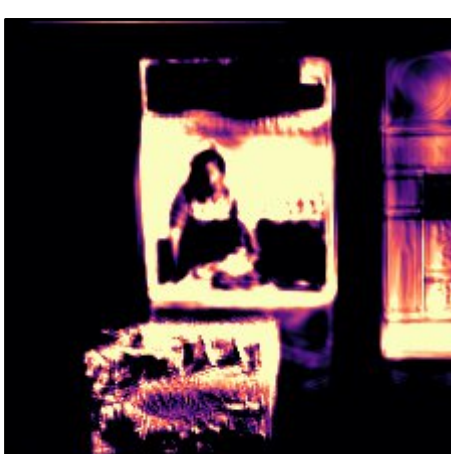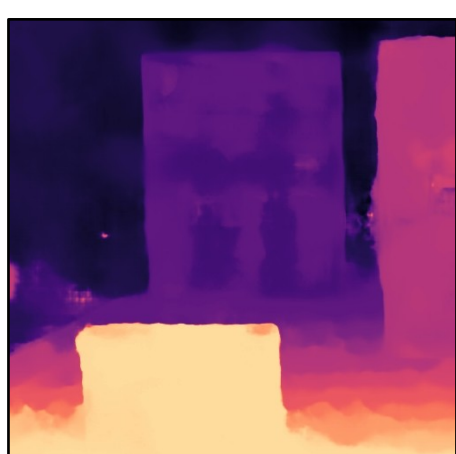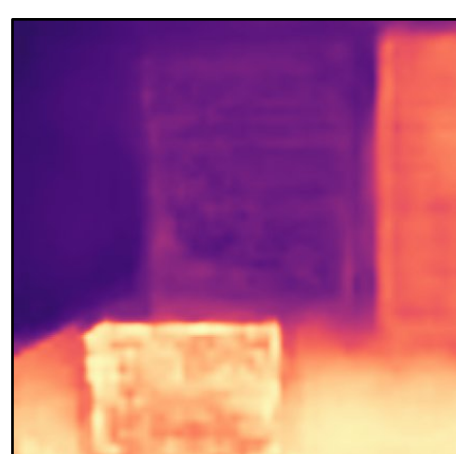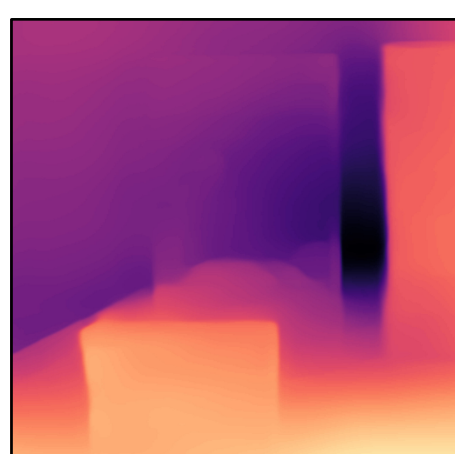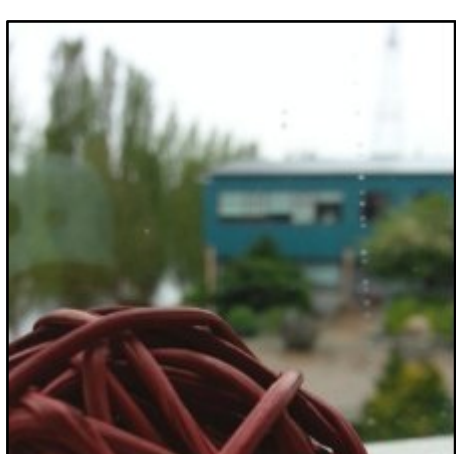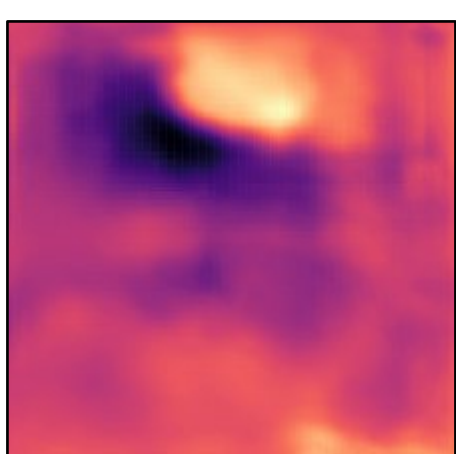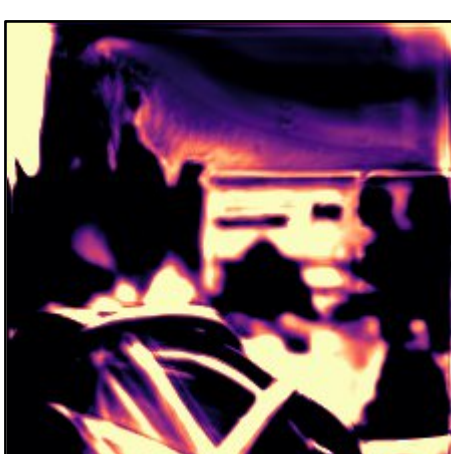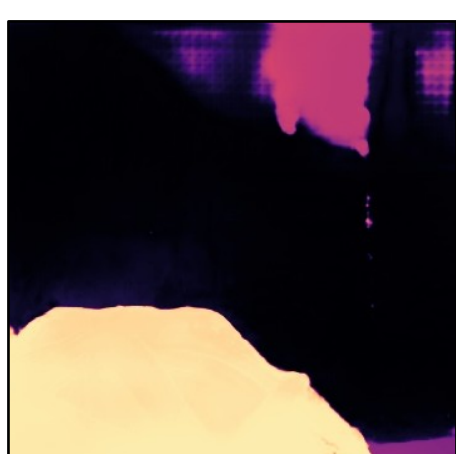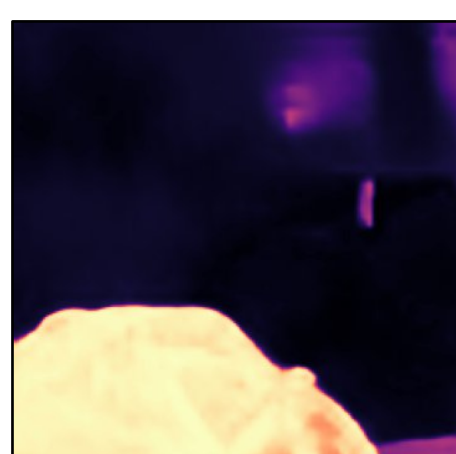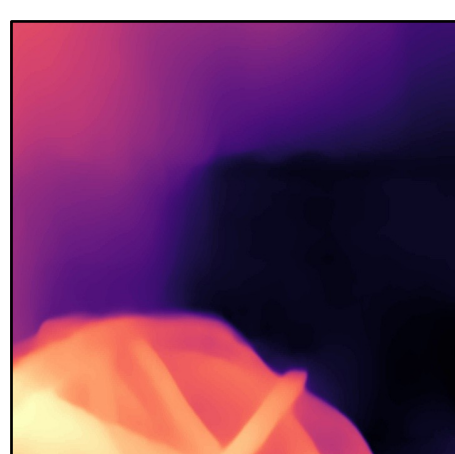



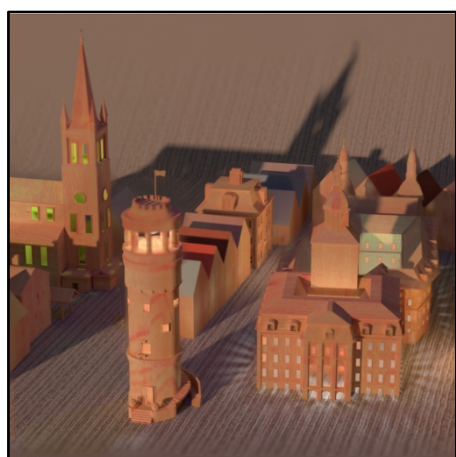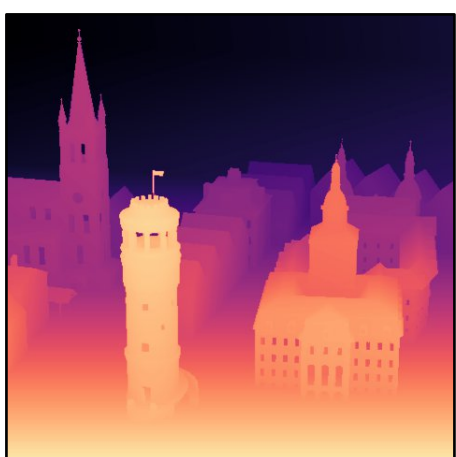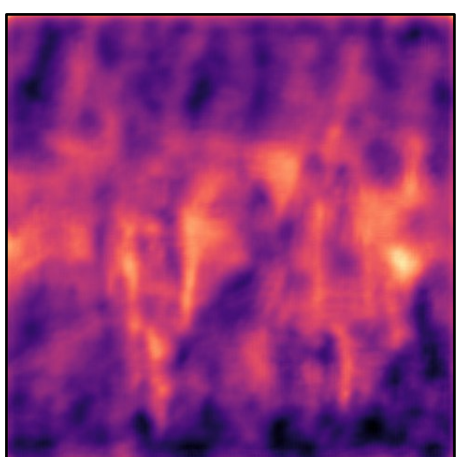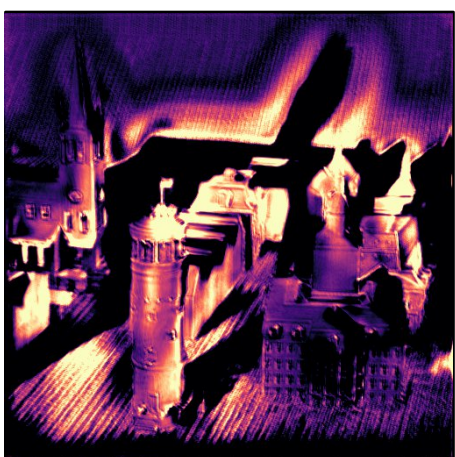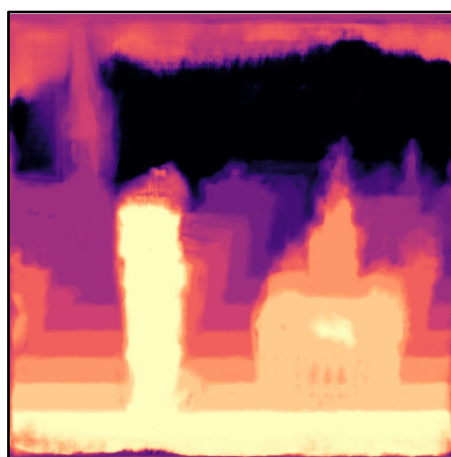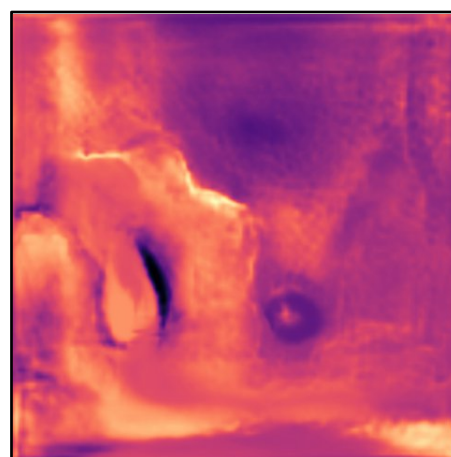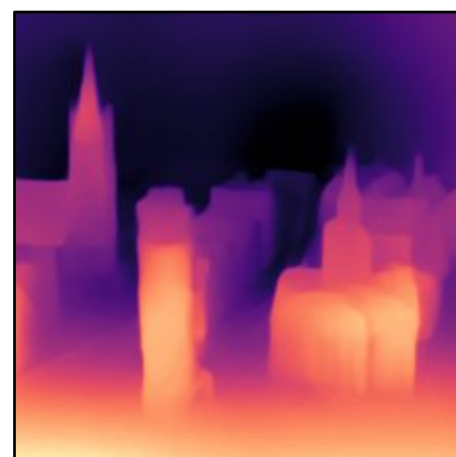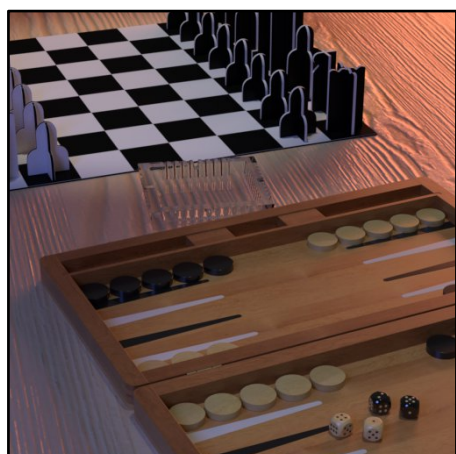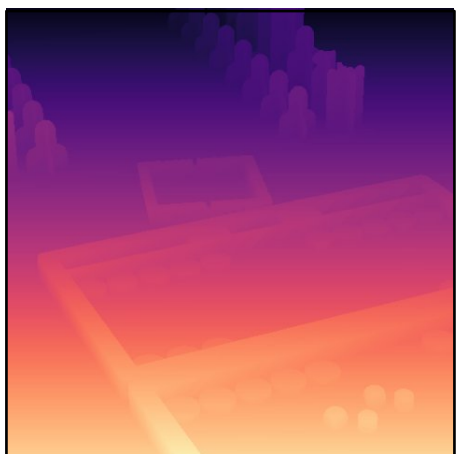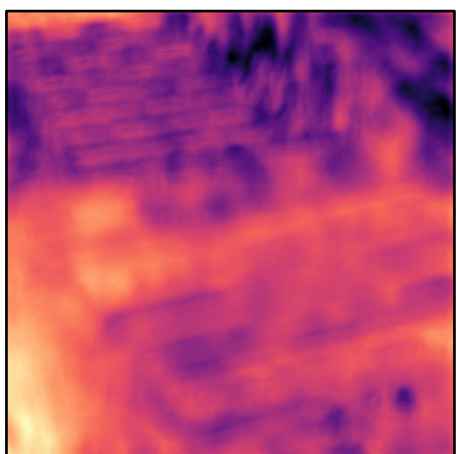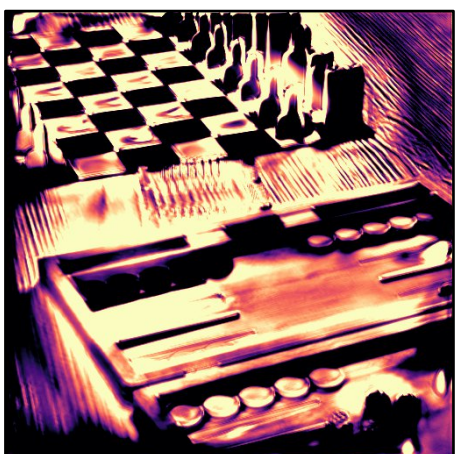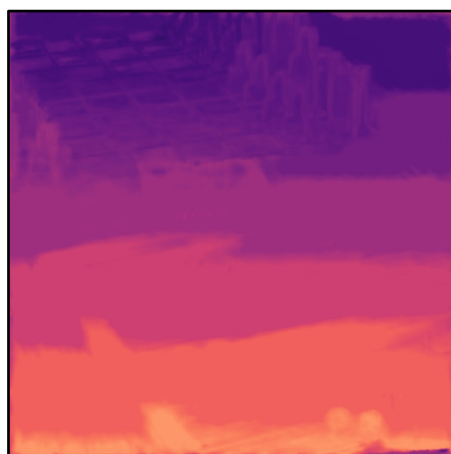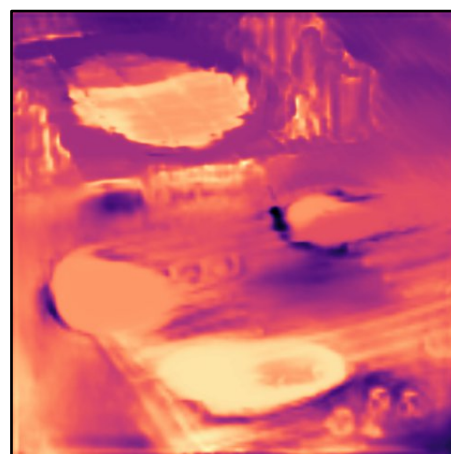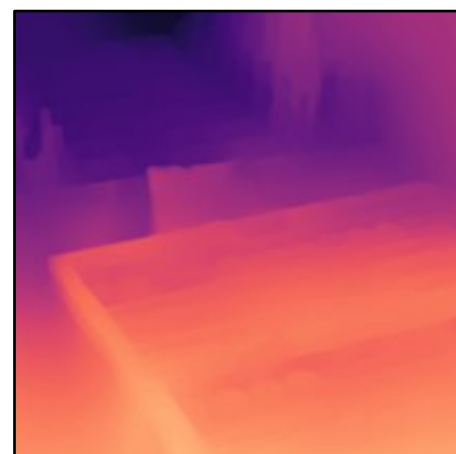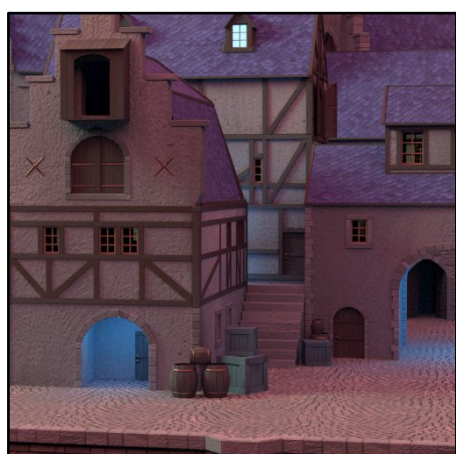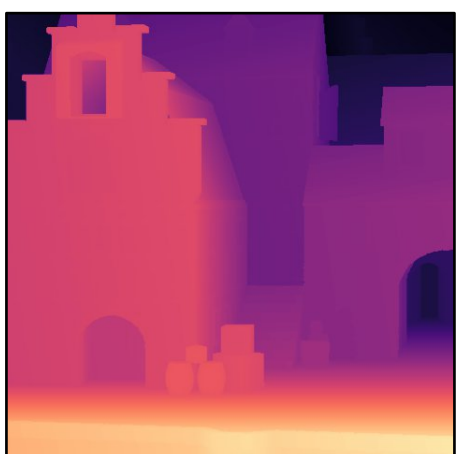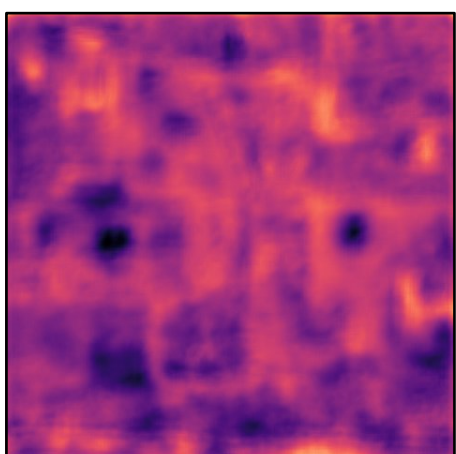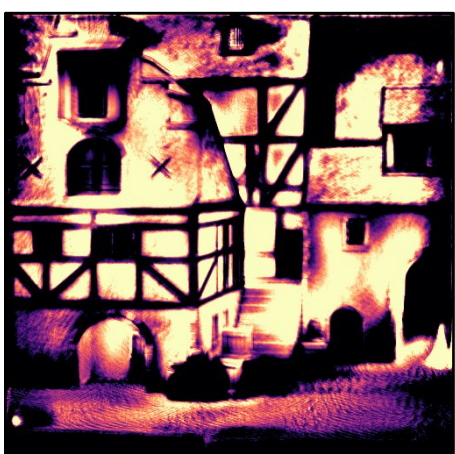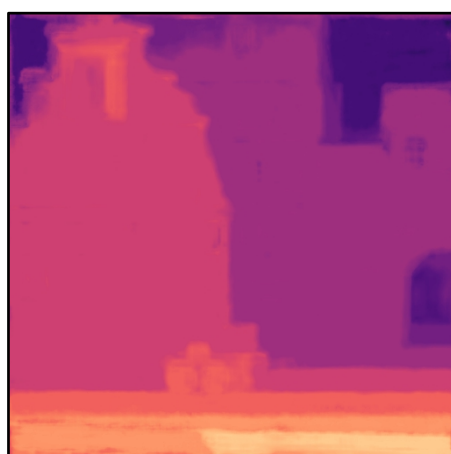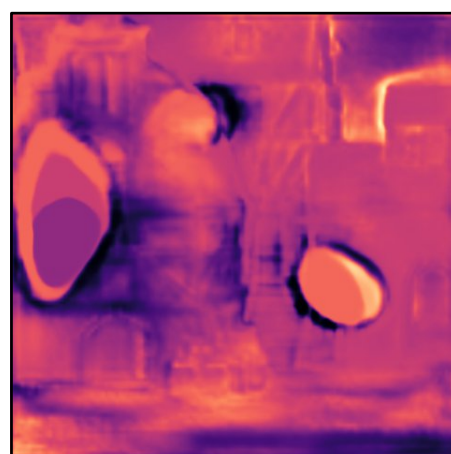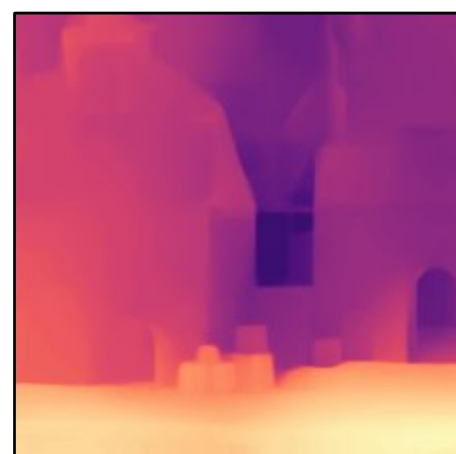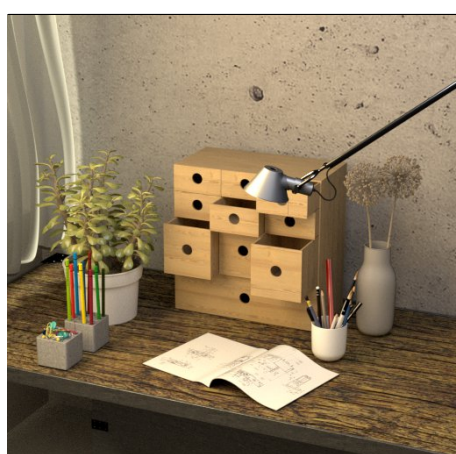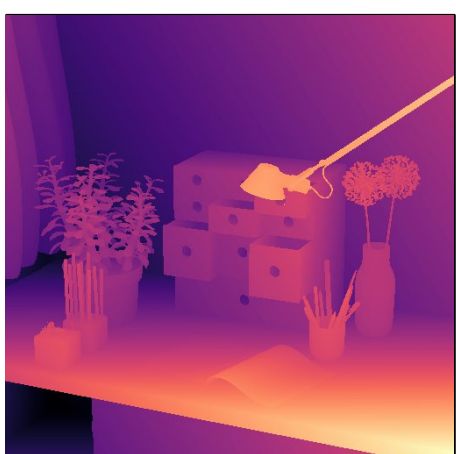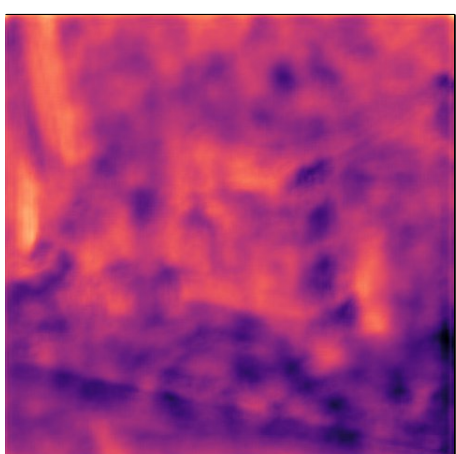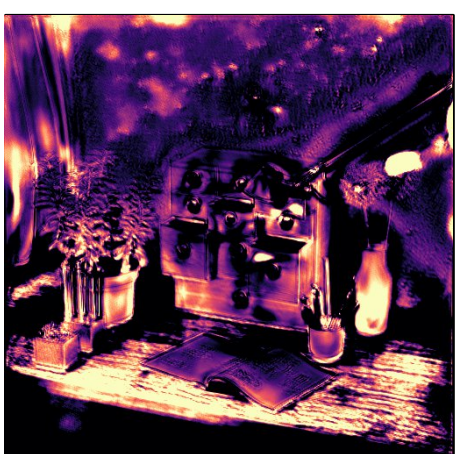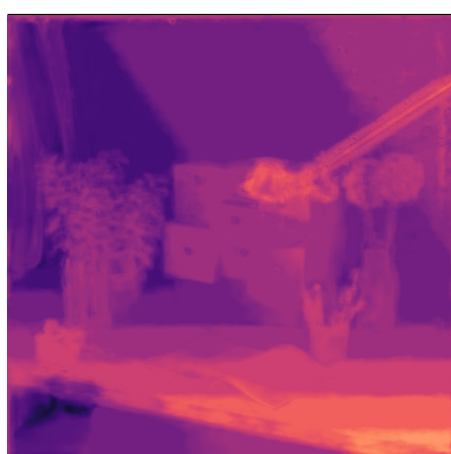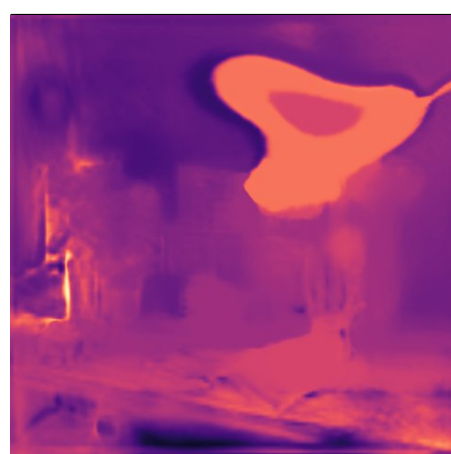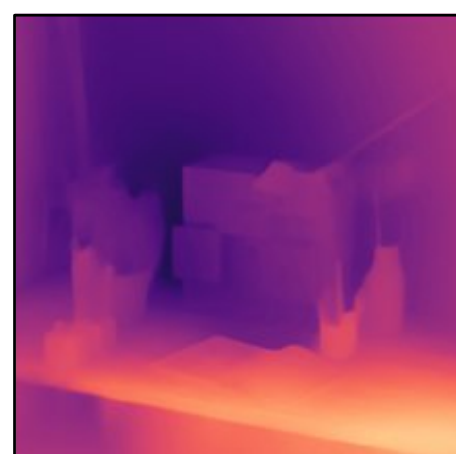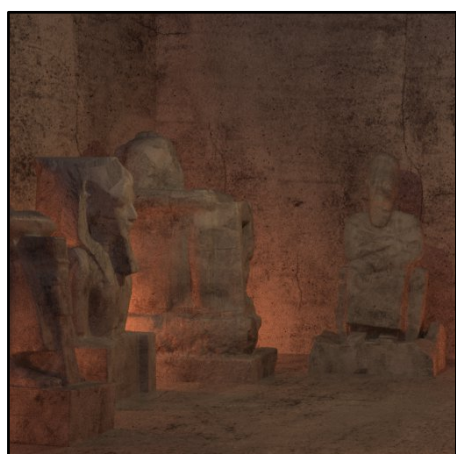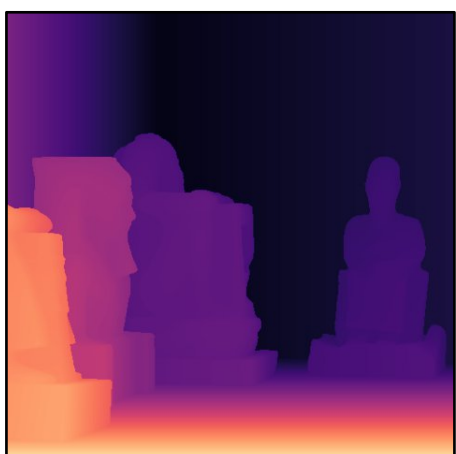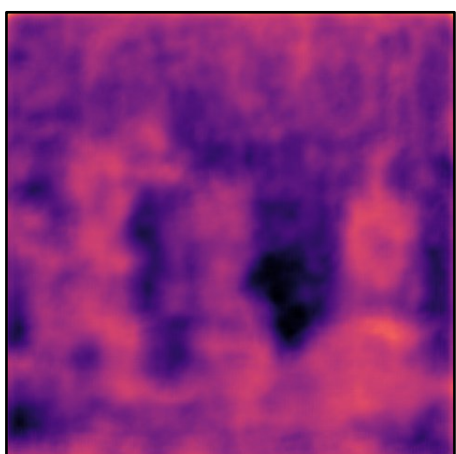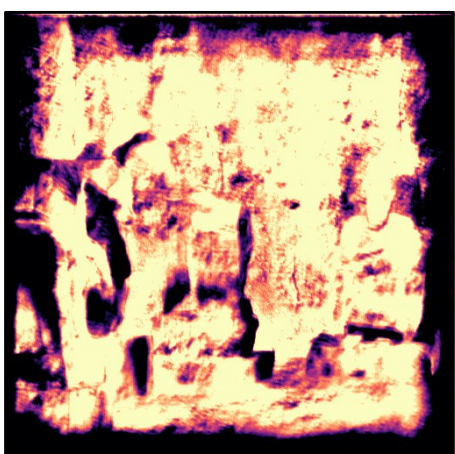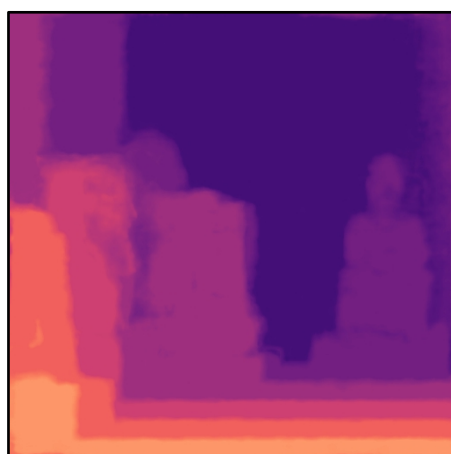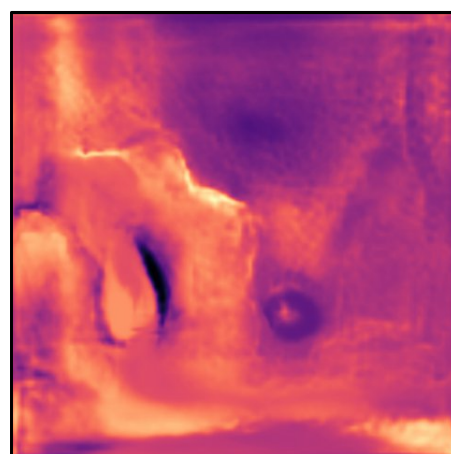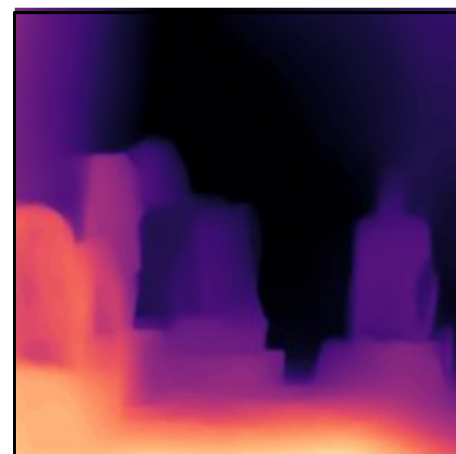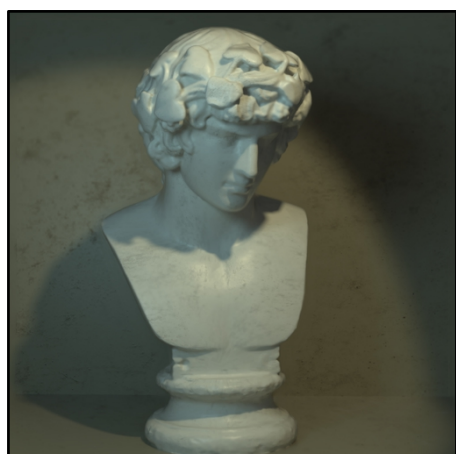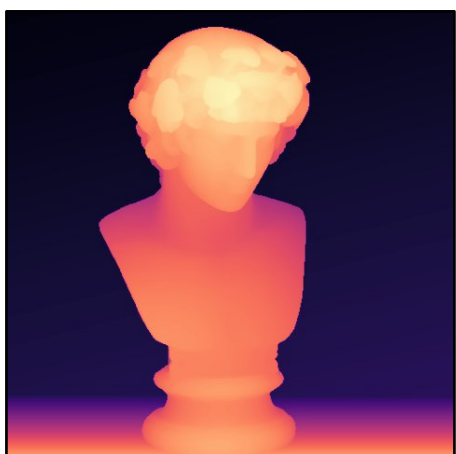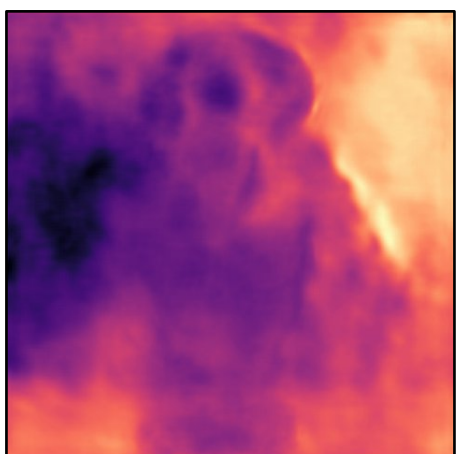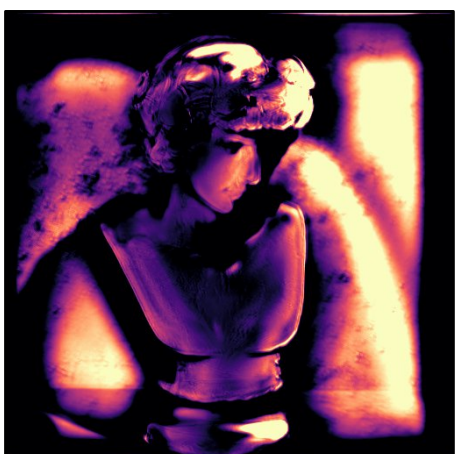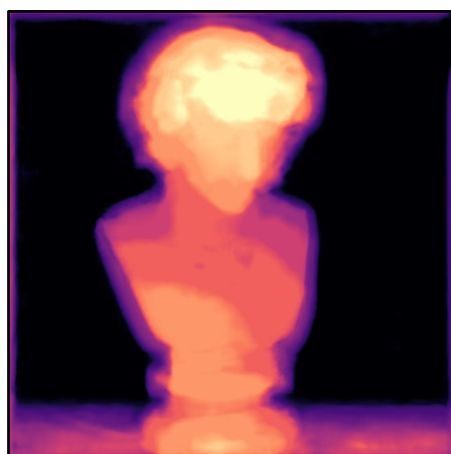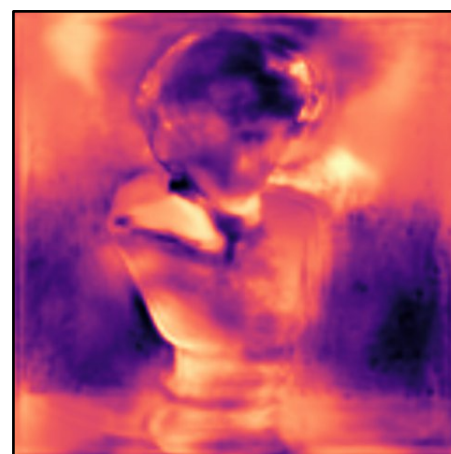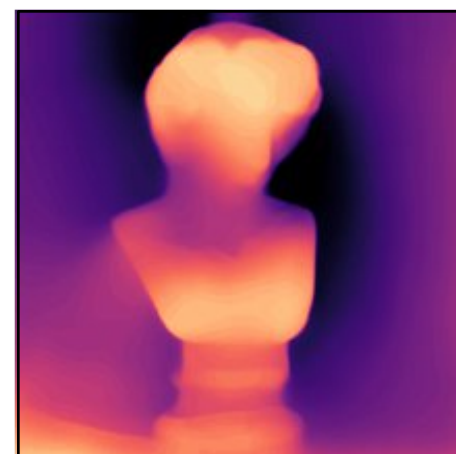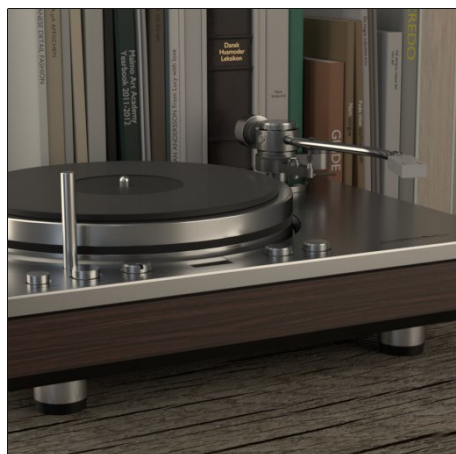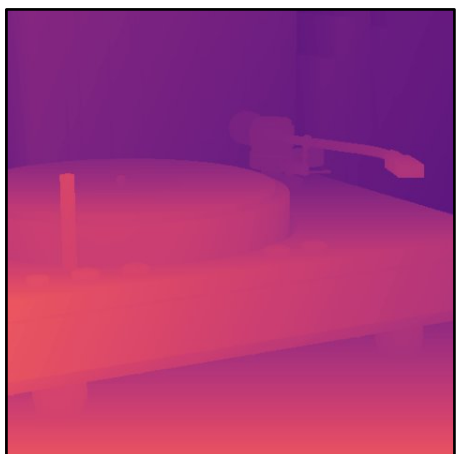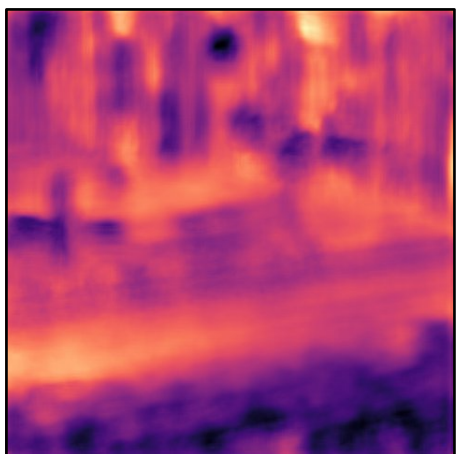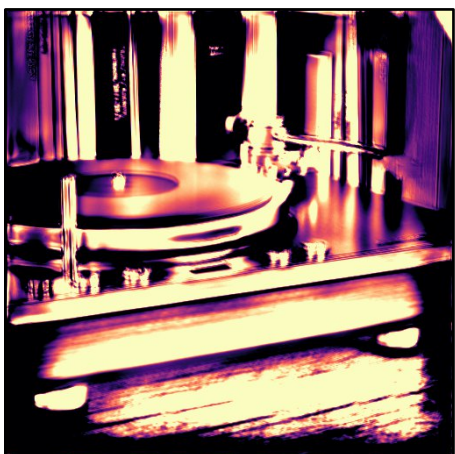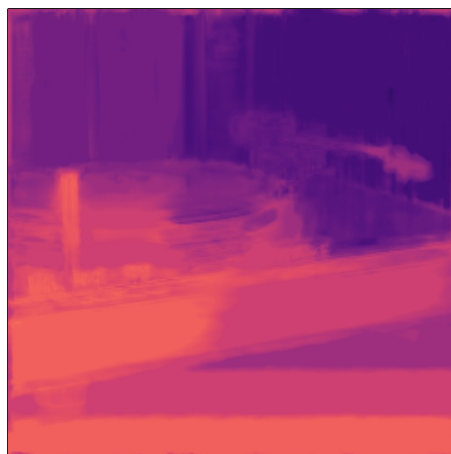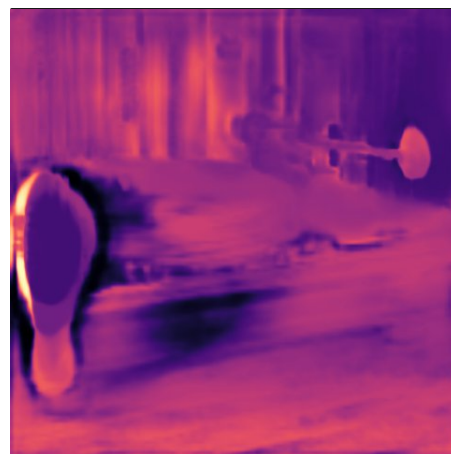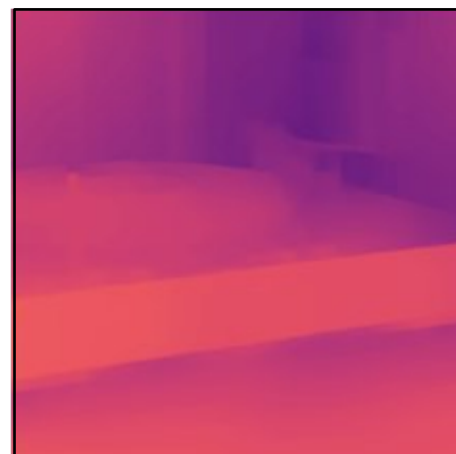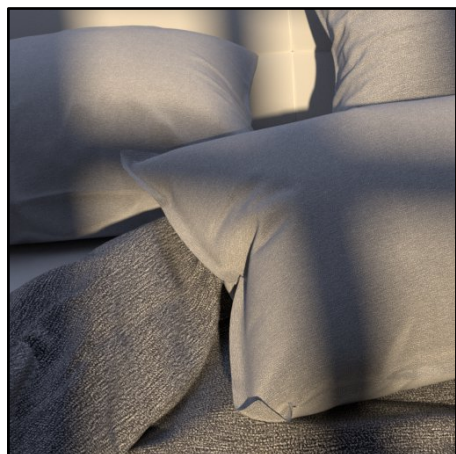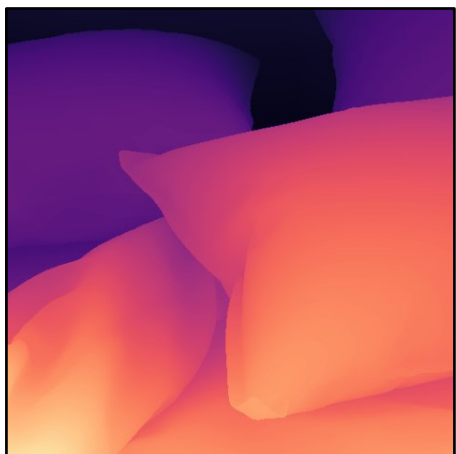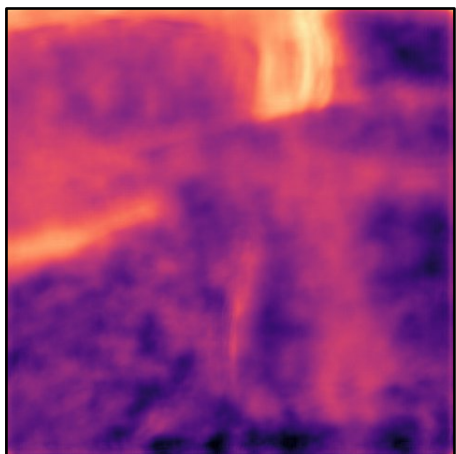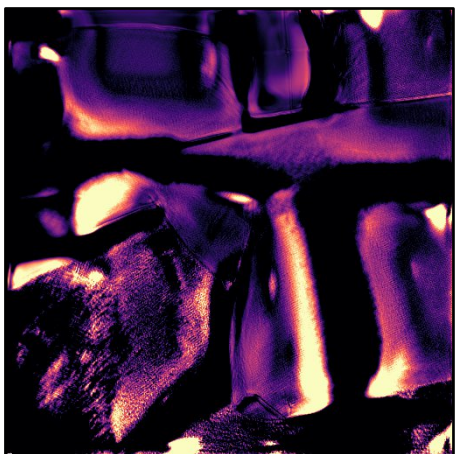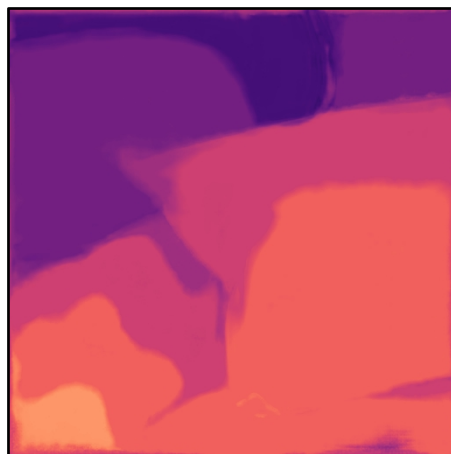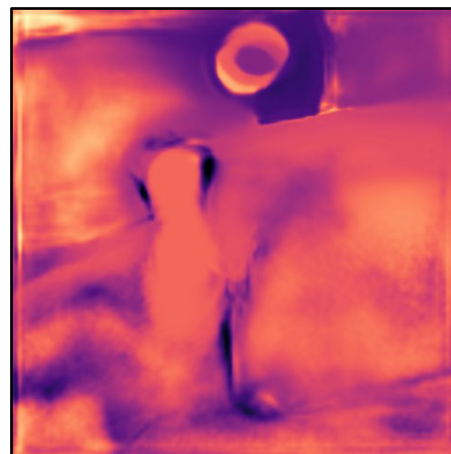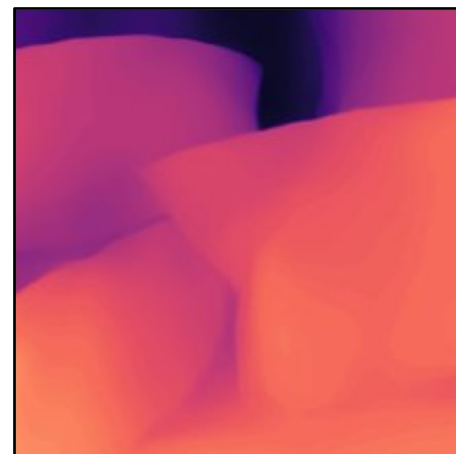



### Early-stage multi-Kernel 2D.

**Box:** input channel, output channel, kernel size, stride  
**Parameter:** (batch size, output channel, height, width).

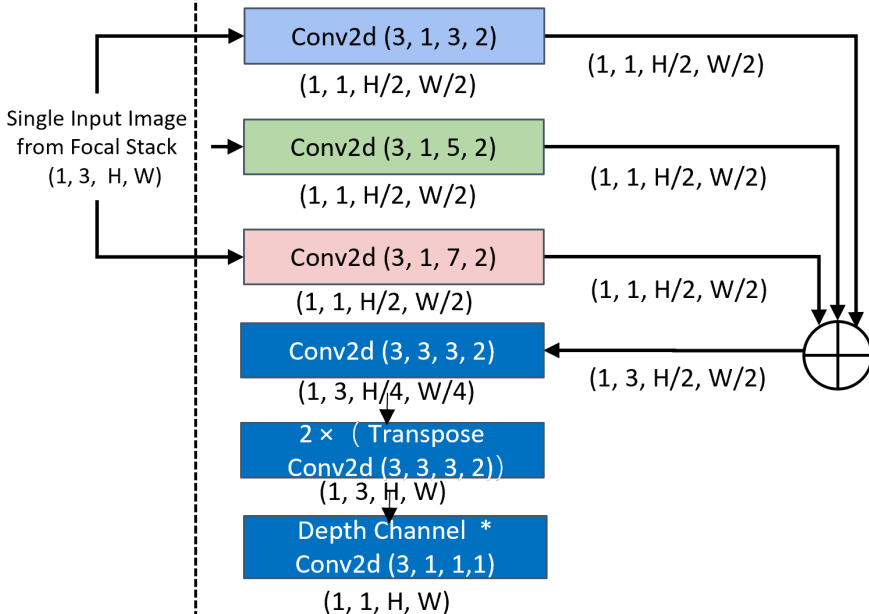

**Transformer encoder + LSTM.**  
**Parameter: (number of tokens, dimension per token).**

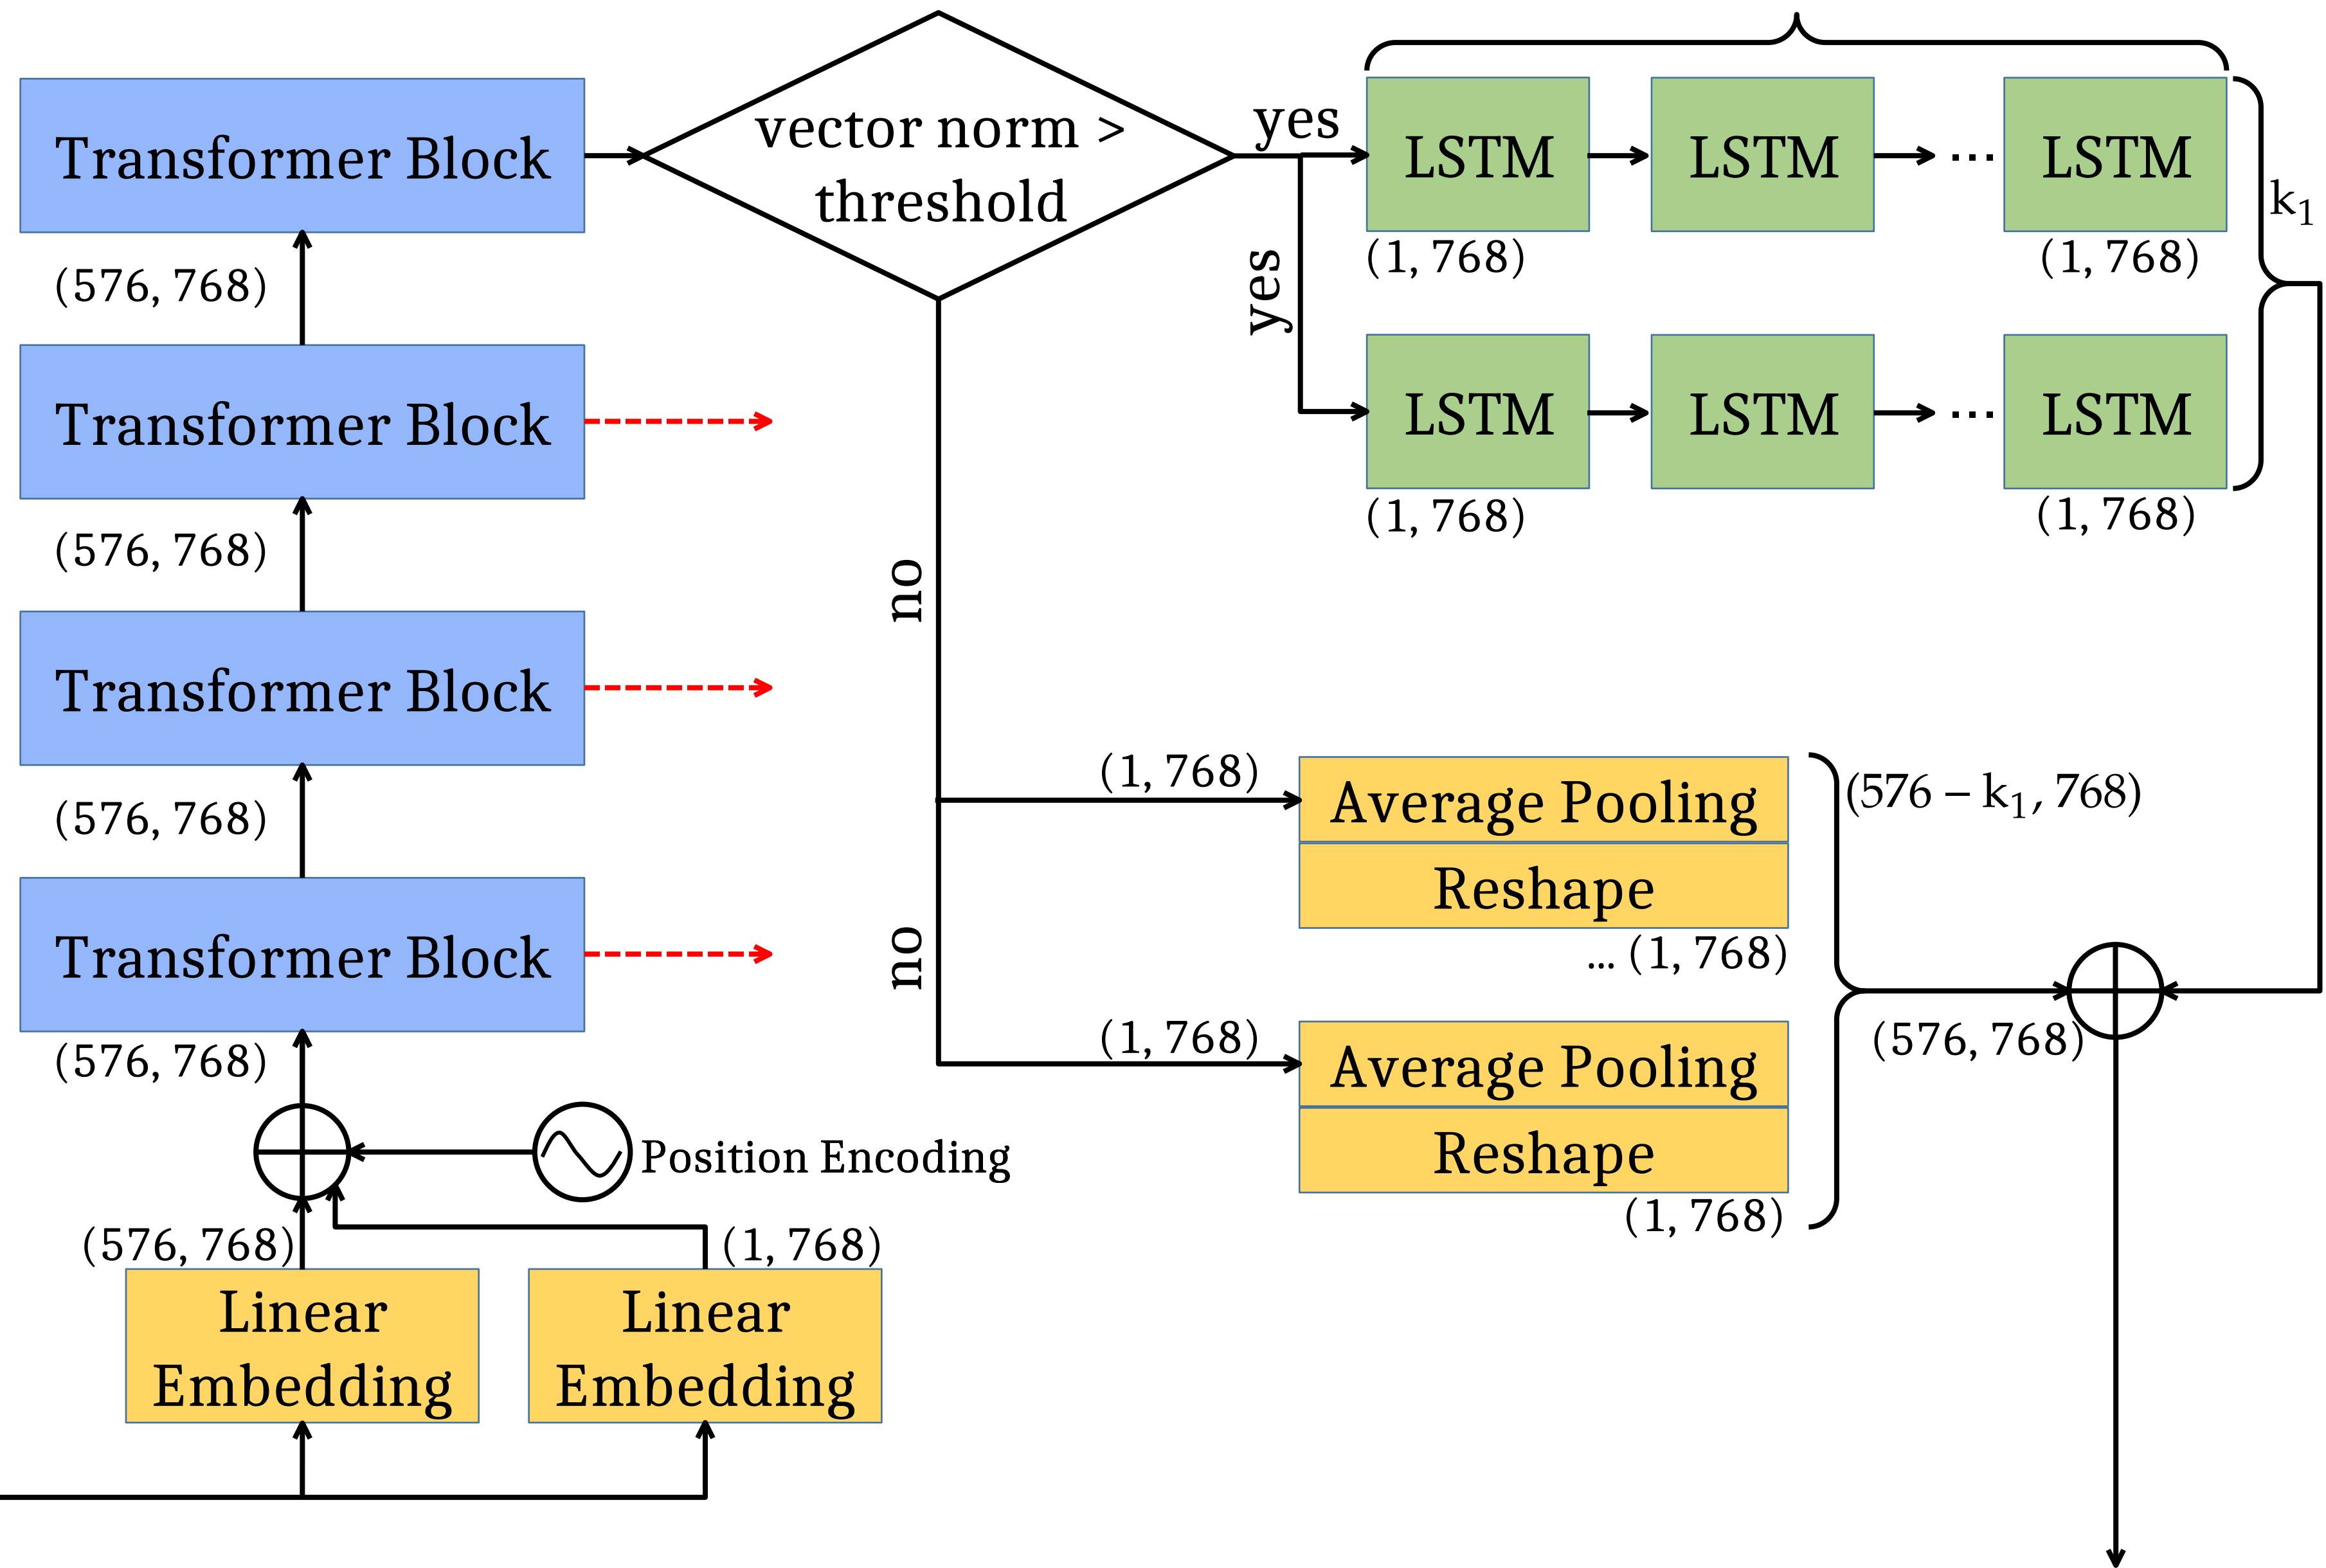

## Decoder: Composition + CNN + Head

Box: input channel, output channel, kernel size.

Parameter: (batch size\*samples, output channel, height, width).

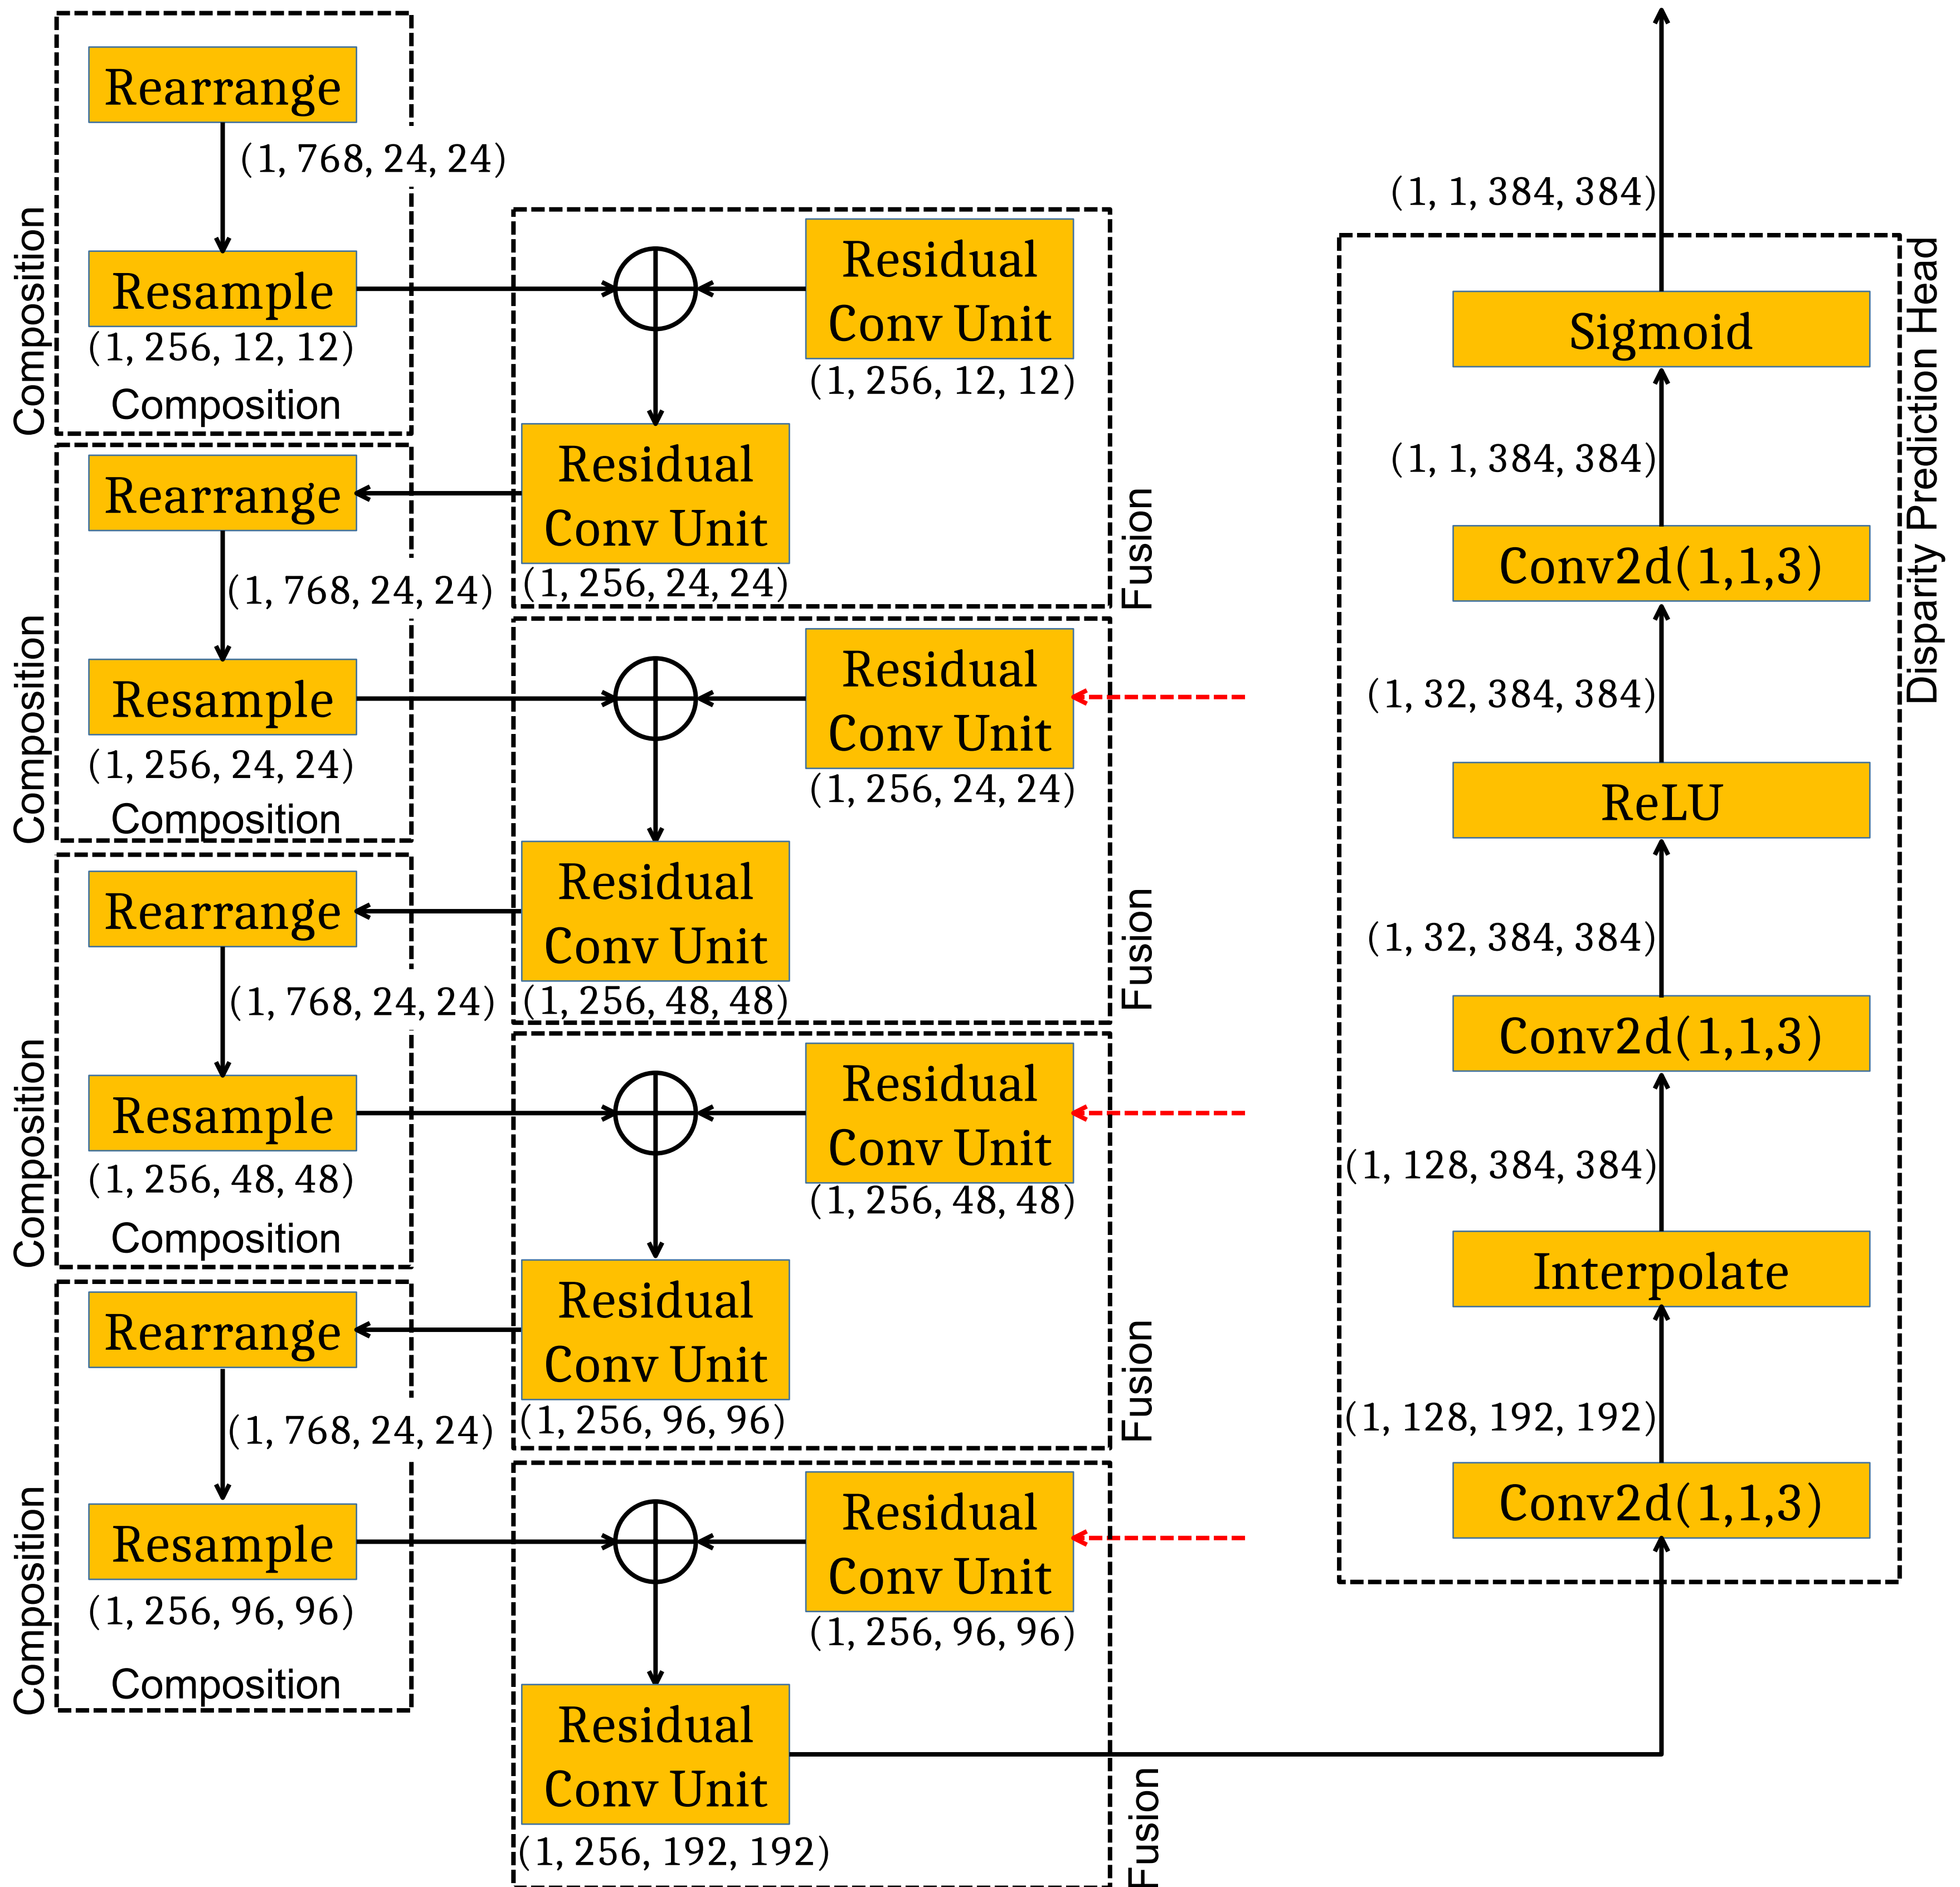

Transformer Block

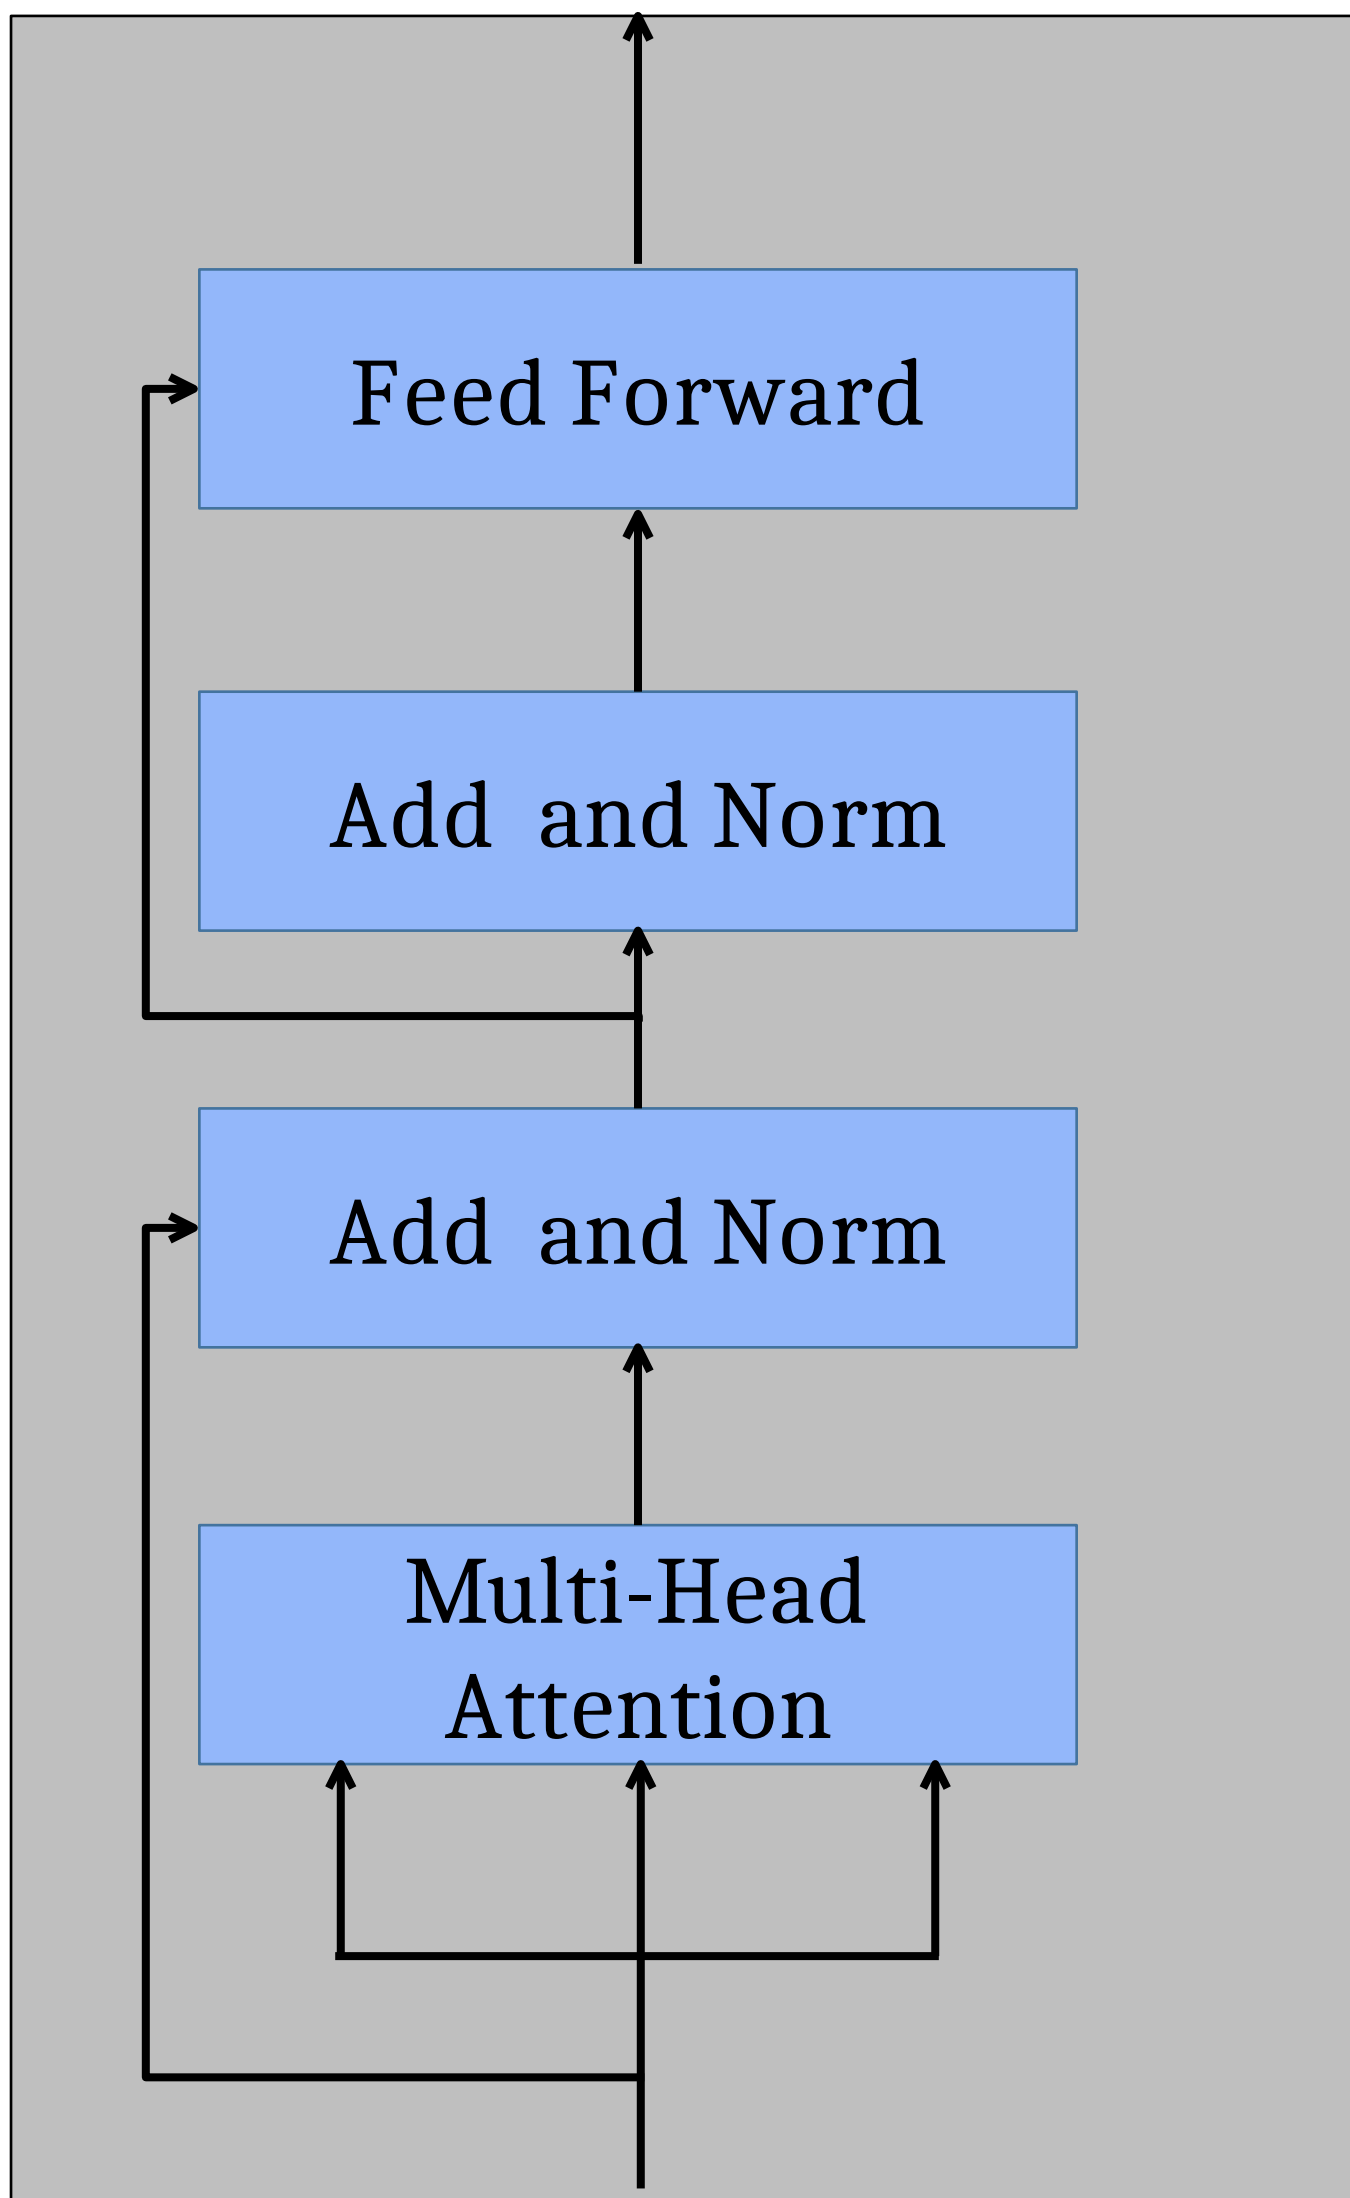

Residual Conv. Unit

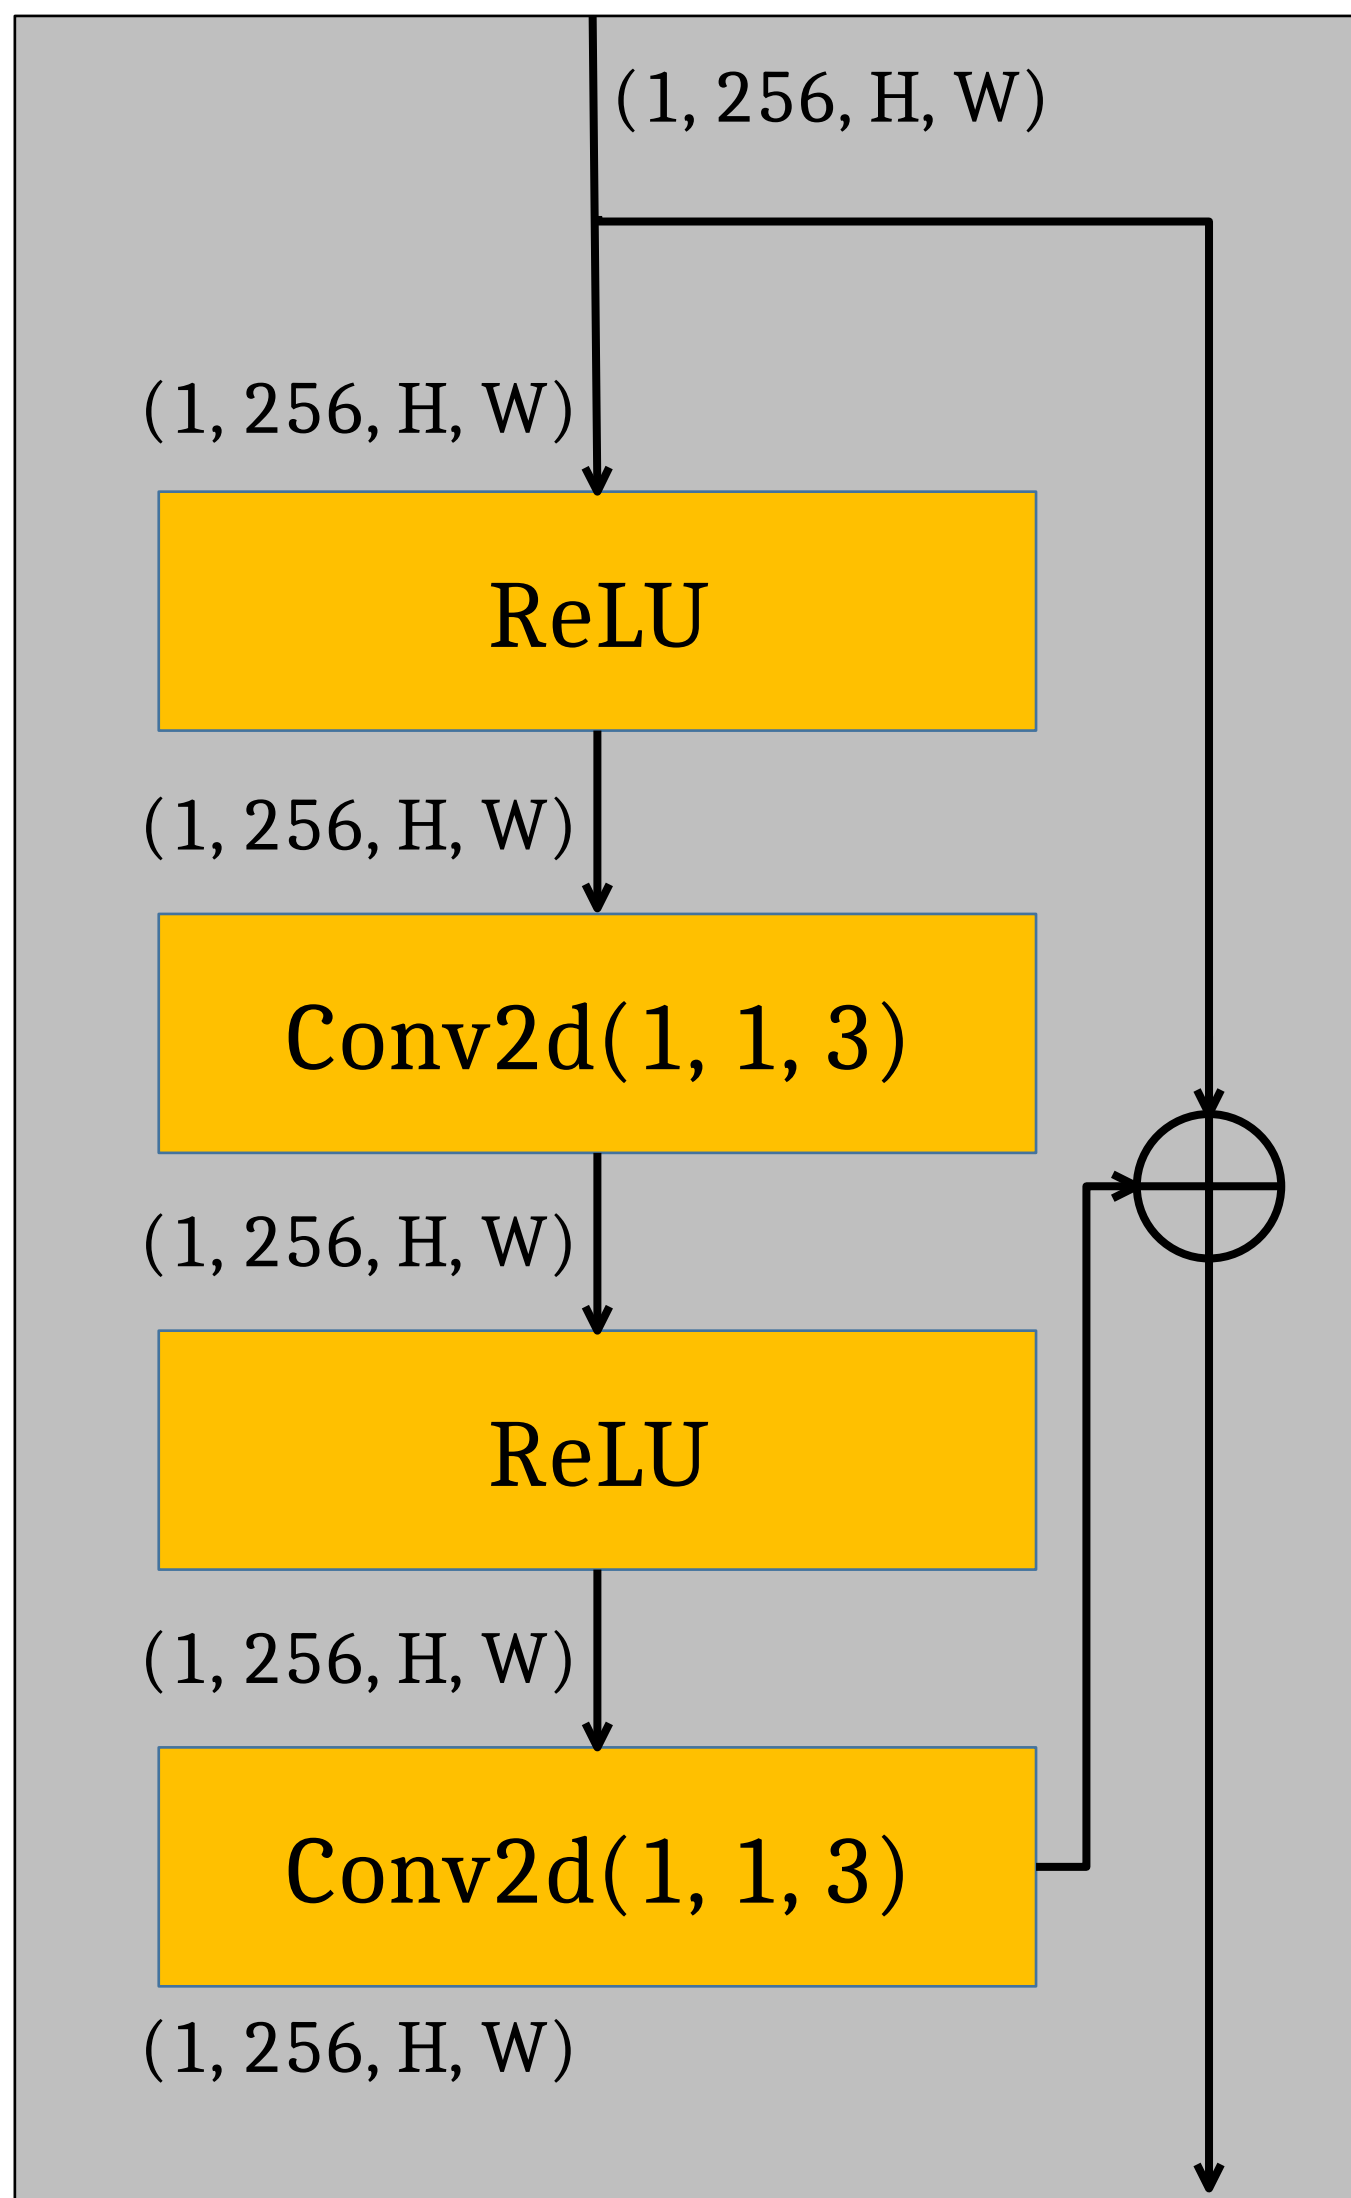



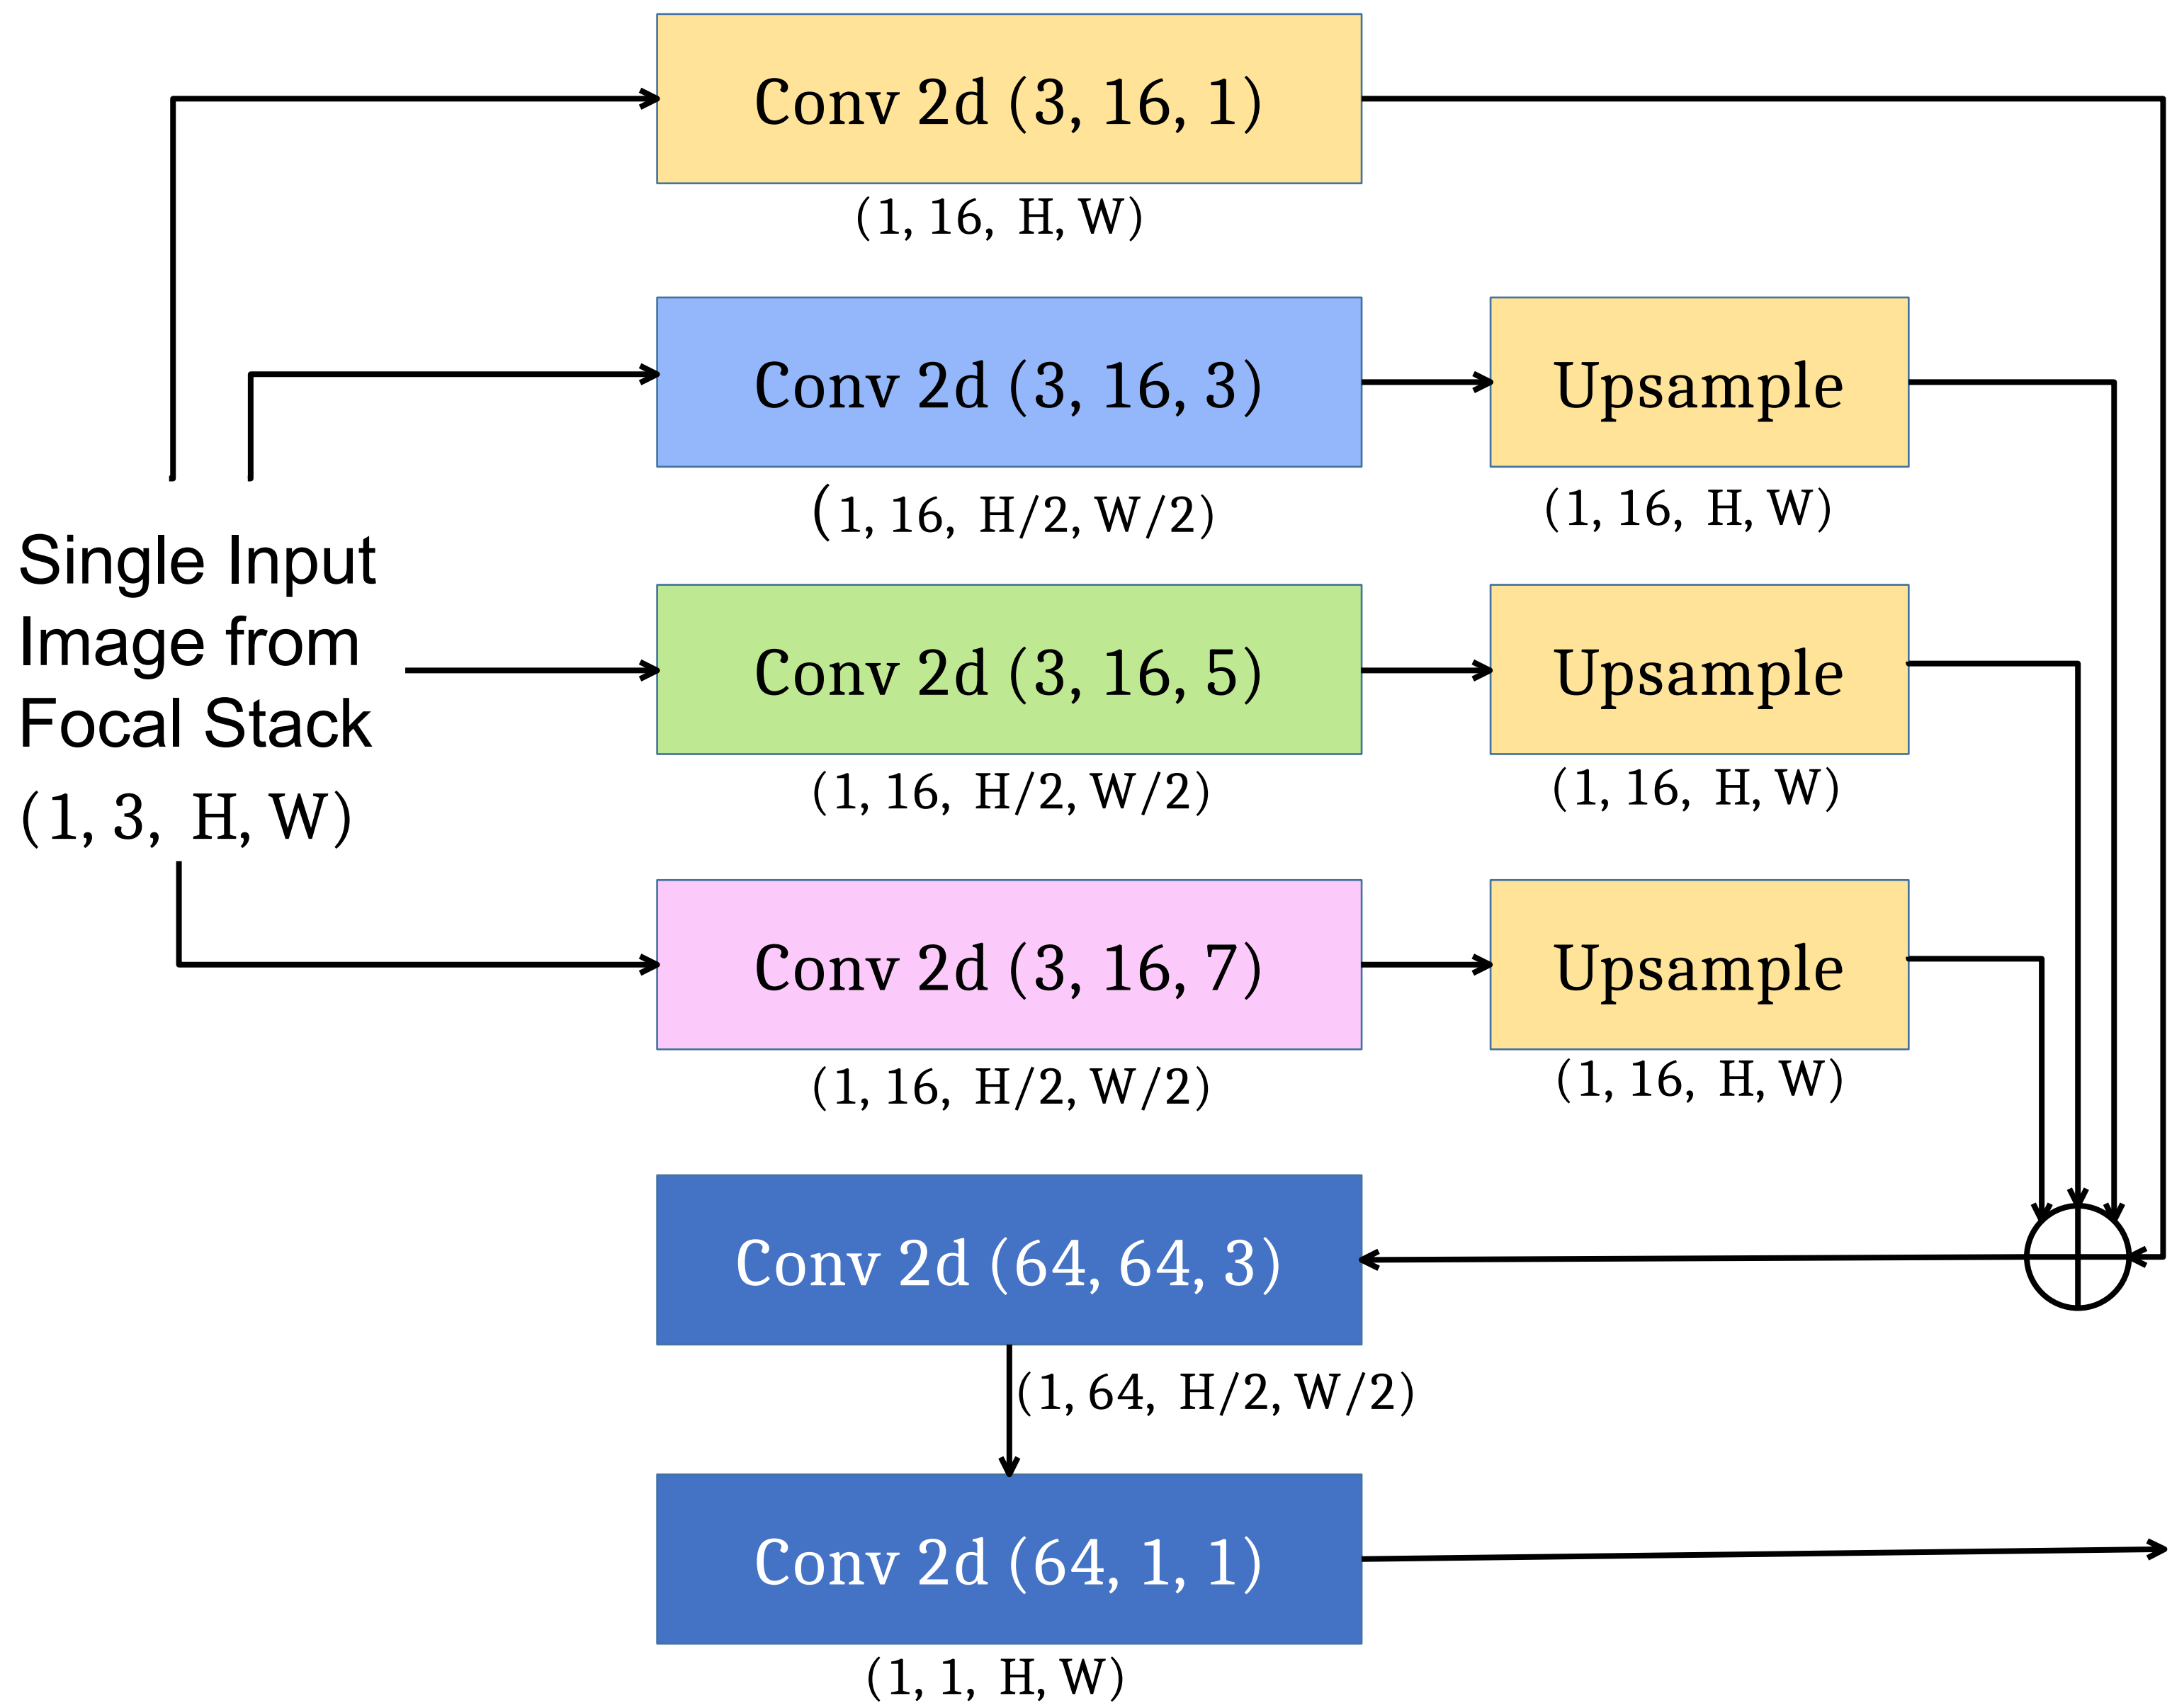



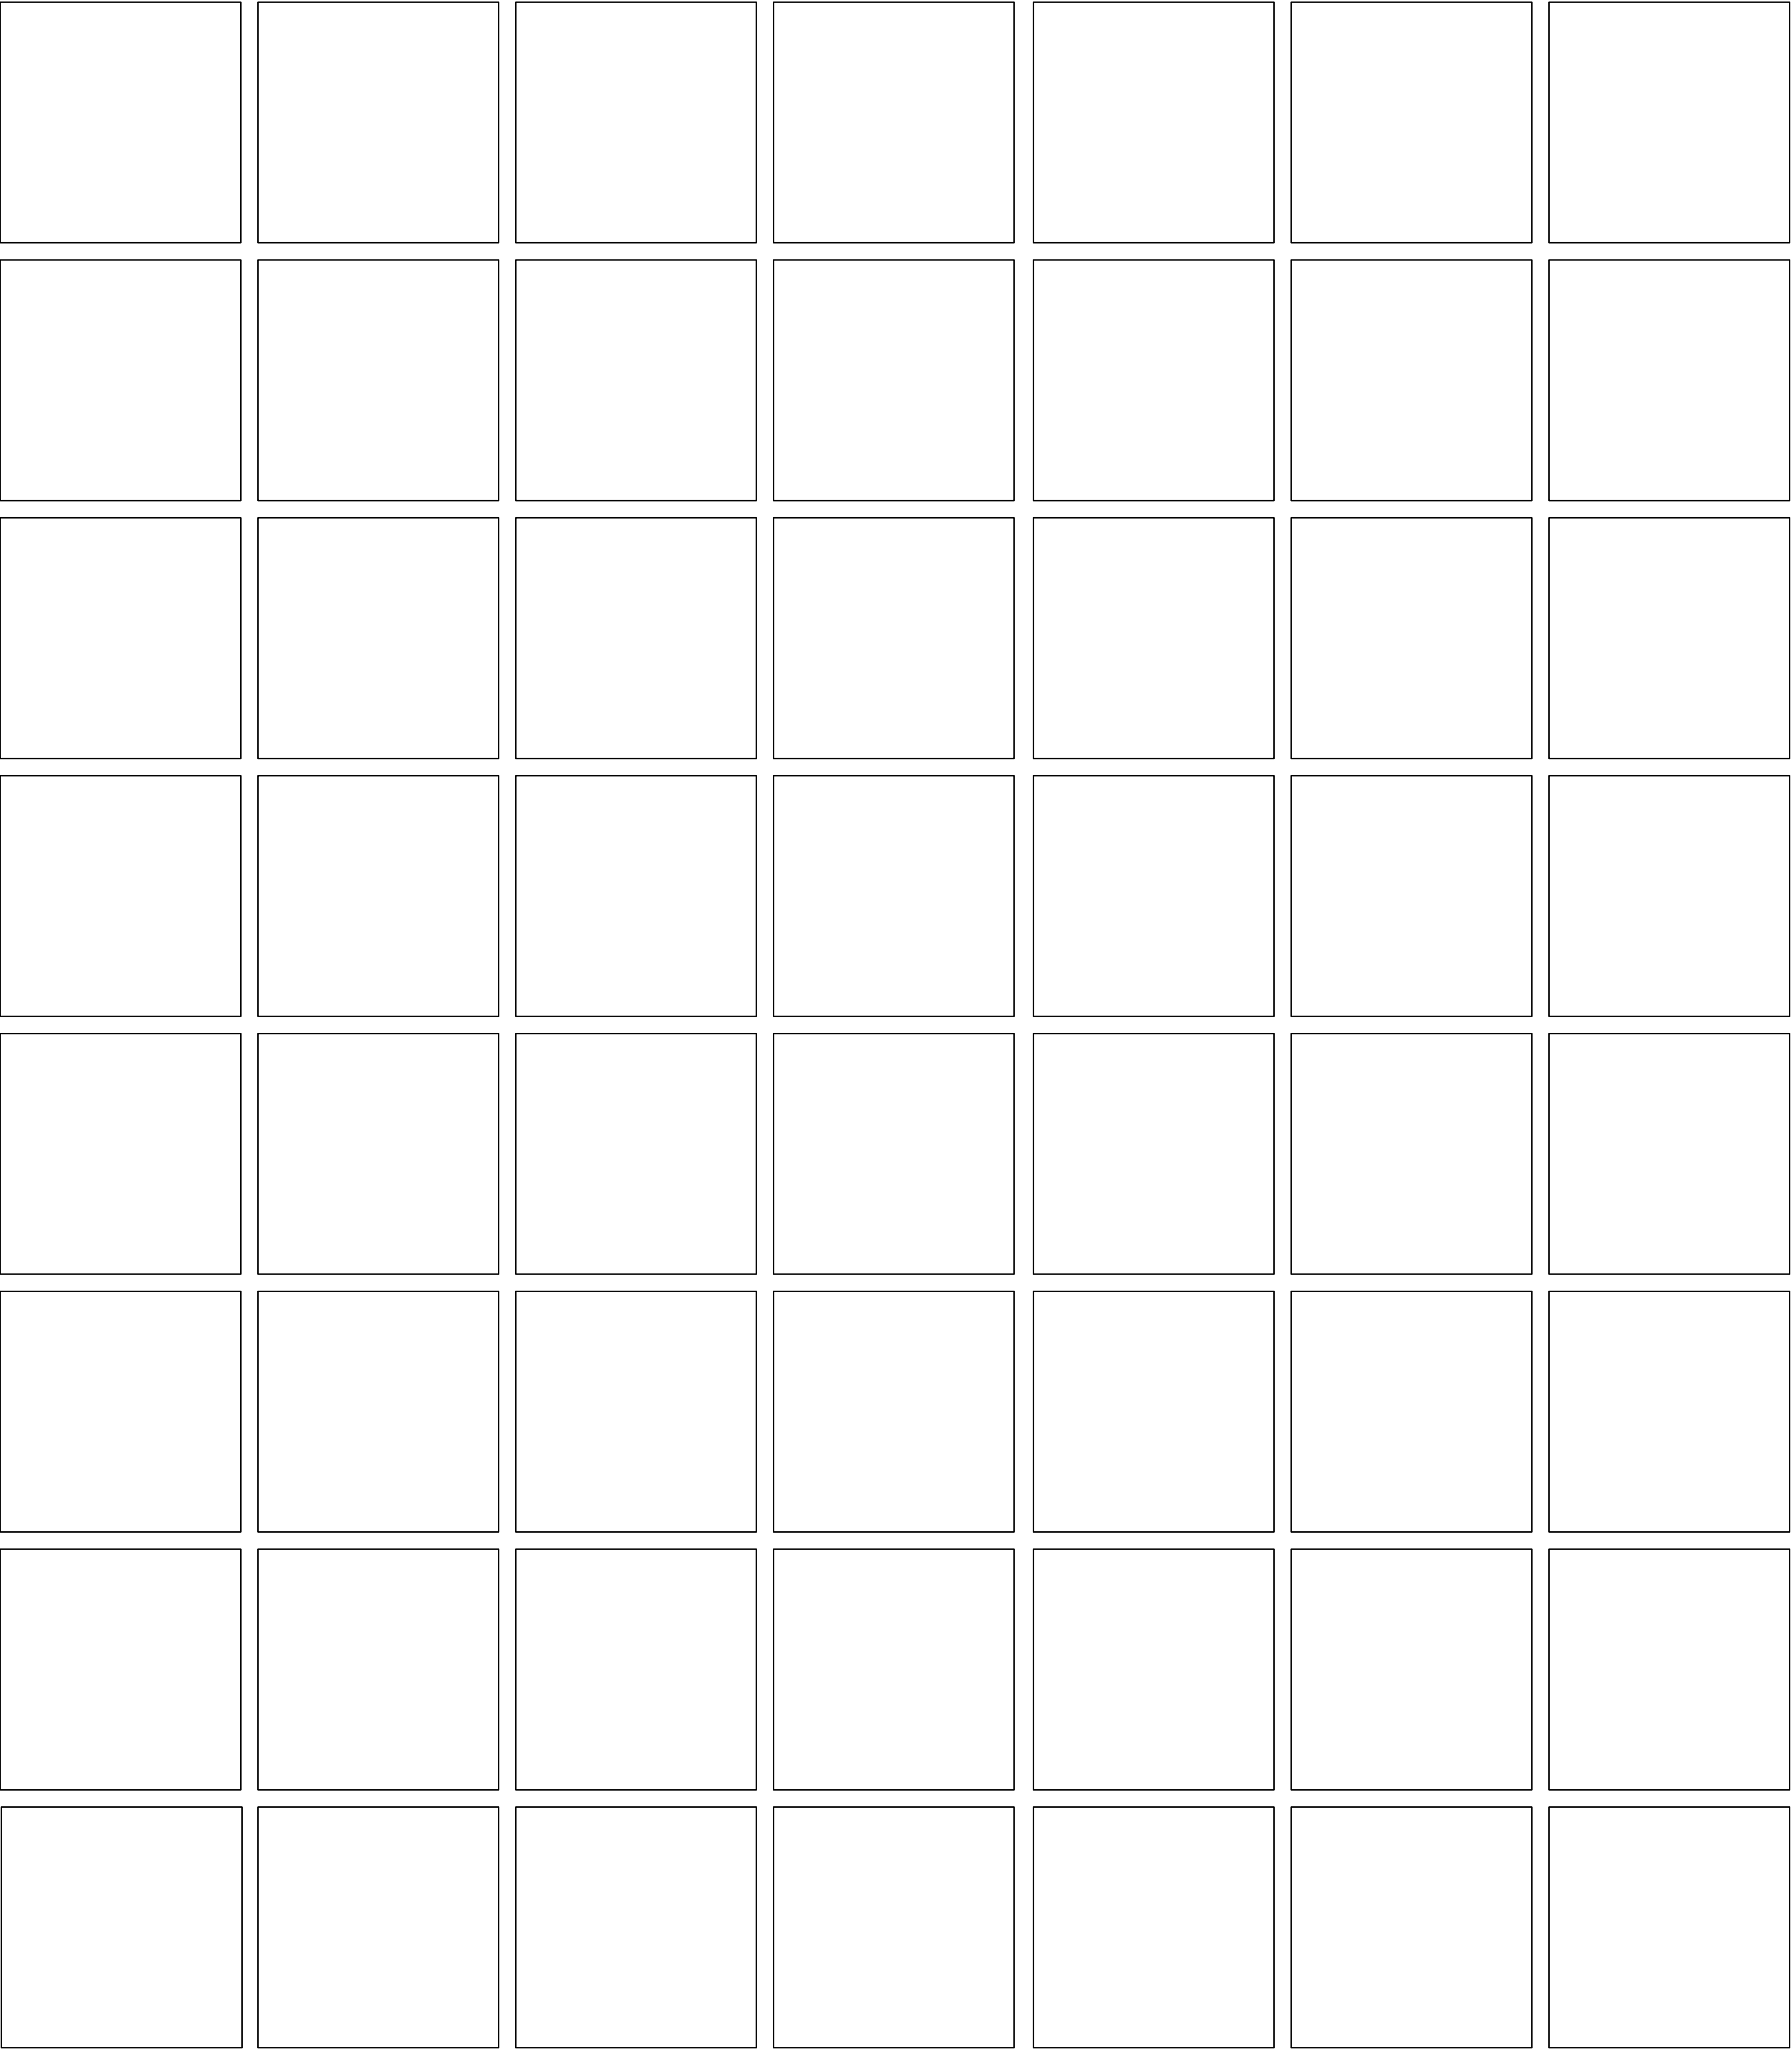

Supplement: Supplementary file 1 [file Presentation1_supplimentary.pdf]
